# Supplementary material for: Electronic friction for a slow impurity in an inhomogeneous metallic system
Source: arXiv:1302.0986 ancillary file (2013-02-05)
Supplement: Supplementary file 1 [file 2013.02.02_Note1.pdf]

## Note 1

Friction coefficient for the Free Electron Gas.  
Relation between the expression of Hellsing and Persson  
and that of the Shifted Fermi Sphere.

A. Salin\*,

12, rue Jules Testaud, 33700 Mérignac, France

February 2, 2013

---

\*Retired from Université de Bordeaux I

The aim of this note is to exhibit the relation between expression (12) of [1] (referred to as HP) and that obtained with the Shifted Fermi Sphere (SFS, see, e.g., [2]). The friction coefficient is the coefficient of the term linear in  $v$ , for  $v \rightarrow 0$  [3], in the expression of the stopping power.

In this note, we use a *collisional* formulation, i.e., we assume that the impurity potential goes to zero at large distances and that the background, in the absence of impurity, has at least a spherical symmetry.

Atomic units are used throughout

# 1 Lemmas

We first derive some mathematical properties that are used in the following discussion.

## 1.1 Generalized microreversibility

Let  $f(\mathbf{k}, \hat{\mathbf{k}}')$  be the transition amplitude for electron scattering by some potential  $V$ , not necessarily spherically symmetric.

$$f(\mathbf{k}, \hat{\mathbf{k}}') = (2\pi)^2 \int d\mathbf{r} [\phi_{\mathbf{k}'}(\mathbf{r})]^* V(\mathbf{r}) \Psi_{\mathbf{k}}^+(\mathbf{r}) \quad (1a)$$

$$= (2\pi)^2 \int d\mathbf{r} [\Psi_{\mathbf{k}'}^-(\mathbf{r})]^* V(\mathbf{r}) \phi_{\mathbf{k}}(\mathbf{r}) \quad (1b)$$

Here,  $\Psi_{\mathbf{k}}^{\pm}(\mathbf{r})$  (+: outgoing, -: ingoing asymptotic condition) is the solution of the Schrödinger equation including the potential  $V(\mathbf{r})$ , and  $\phi_{\mathbf{k}}(\mathbf{r})$  is the solution in the absence of  $V(\mathbf{r})$ . The well known microreversibility relation reads:

$$f(\mathbf{k}, \hat{\mathbf{k}}') = f(-\mathbf{k}', -\hat{\mathbf{k}}) \quad (2)$$

It arises from the simple properties:

$$\Psi_{\mathbf{k}}^-(\mathbf{r}) = [\Psi_{-\mathbf{k}}^+(\mathbf{r})]^* \quad ; \quad \phi_{\mathbf{k}}(\mathbf{r}) = [\phi_{-\mathbf{k}}(\mathbf{r})]^* \quad (3)$$

For  $k=k'$ , this property is satisfied by any matrix element, say  $F(\mathbf{k}, \hat{\mathbf{k}}')$ , of a hermitic operator, say  $\mathcal{O}$ , between scattering functions, say  $\Psi_{\mathbf{k}}^{\pm}(\mathbf{r})$  and  $\Phi_{\mathbf{k}}^{\pm}(\mathbf{r})$ :

$$F(\mathbf{k}, \hat{\mathbf{k}}') = \langle \Phi_{\mathbf{k}'}^- | \mathcal{O} | \Psi_{\mathbf{k}}^+ \rangle \quad (4)$$

*provided* a condition similar to the equality between (1a) and (1b) prevails:

$$\langle \Phi_{\mathbf{k}'}^- | \mathcal{O} | \Psi_{\mathbf{k}}^+ \rangle = \langle \Psi_{\mathbf{k}'}^- | \mathcal{O} | \Phi_{\mathbf{k}}^+ \rangle \quad (5)$$

The latter condition is satisfied whenever we invoke microreversibility in the following discussion.

## 1.2 Lemma 1

Consider the integral:

$$\mathcal{J} = \int d\hat{\mathbf{k}} \int d\hat{\mathbf{k}}' [\hat{\mathbf{v}} \cdot (\hat{\mathbf{k}} - \hat{\mathbf{k}}')] [F^I(\mathbf{k}, \hat{\mathbf{k}}')]^* F^{II}(\mathbf{k}, \hat{\mathbf{k}}') \quad (6)$$

where  $F^I$  and  $F^{II}$  are any amplitude satisfying (2). Then, defining  $\theta_k = \arccos(\hat{\mathbf{v}} \cdot \hat{\mathbf{k}})$ ,

$$\mathcal{J} = \int d\hat{\mathbf{k}} \cos \theta_k \int d\hat{\mathbf{k}}' \left\{ [F^I(\mathbf{k}, \hat{\mathbf{k}}')]^* F^{II}(\mathbf{k}, \hat{\mathbf{k}}') - [F^I(\mathbf{k}', \hat{\mathbf{k}})]^* F^{II}(\mathbf{k}', \hat{\mathbf{k}}) \right\} \quad (7a)$$

$$= \int d\hat{\mathbf{k}} \cos \theta_k \int d\hat{\mathbf{k}}' \left\{ [F^I(\mathbf{k}, \hat{\mathbf{k}}')]^* F^{II}(\mathbf{k}, \hat{\mathbf{k}}') - [F^I(-\mathbf{k}, -\hat{\mathbf{k}}')]^* F^{II}(-\mathbf{k}, -\hat{\mathbf{k}}') \right\} \quad (7b)$$

$$= \int d\hat{\mathbf{k}} \cos \theta_k \int d\hat{\mathbf{k}}' \left\{ [F^I(\mathbf{k}, \hat{\mathbf{k}}')]^* F^{II}(\mathbf{k}, \hat{\mathbf{k}}') + [F^I(-\mathbf{k}, \hat{\mathbf{k}}')]^* F^{II}(-\mathbf{k}, \hat{\mathbf{k}}') \right\} \quad (7c)$$

$$= 0 \quad (7d)$$

The last step follows from the odd character of the integrand when  $\theta_k$  is changed into  $\pi - \theta_k$ . The property is obviously verified as well when  $F^I = F^{II}$ .

## 1.3 Lemma 2

Let  $f(\mathbf{k}, \hat{\mathbf{k}}')$  be the transition amplitude defined in (1). Consider the integral:

$$\mathcal{J}' = \int d\hat{\mathbf{k}} \int d\hat{\mathbf{k}}' |f(\mathbf{k}, \hat{\mathbf{k}}')|^2 \quad (8)$$

We first use the optical theorem to calculate the integral over  $\hat{\mathbf{k}}'$ :

$$\int d\hat{\mathbf{k}}' |f(\mathbf{k}, \hat{\mathbf{k}}')|^2 = \frac{4\pi}{k} \text{Im}[f(\mathbf{k}, \hat{\mathbf{k}})] \quad (9)$$

As  $f(\mathbf{k}, \hat{\mathbf{k}}) = f(-\mathbf{k}, -\hat{\mathbf{k}})$  (microreversibility), the integral over  $\mathbf{k}$  is zero.

$$\mathcal{J}' = 0 \quad (10)$$

## 2 Friction coefficient from the SFS

We start with expressions (32) and (33) of [4]:

$$\frac{dE}{dZ} = \frac{1}{4\pi^3} \int^{\text{SFS}} d\mathbf{k} k^2 \sigma_v^{\text{tr}} \quad (11)$$

SFS means *shifted Fermi sphere* (Figure 1), i.e., this expression is obtained when working in the moving impurity frame. In the latter frame, the adiabatic approximation leads to a static problem.

$$\sigma_v^{\text{tr}} = \int d\hat{\mathbf{k}}' \hat{\mathbf{v}} \cdot (\hat{\mathbf{k}} - \hat{\mathbf{k}}') |f(\mathbf{k}, \hat{\mathbf{k}}')|^2 \quad (12)$$

Here, the potential  $V$  in (1) is the Kohn-Sham (KS) potential determined self consistently for the *moving* atom [4] and the function  $\Psi_{\mathbf{k}}^+$  is the KS orbital associated with the potential

$V$ , as calculated in [4]. The function  $\phi_{\mathbf{k}'}$  is the unperturbed function, i.e., in the absence of impurity (plane-wave for a jellium). Both functions are normalized on the  $\mathbf{k}$ -scale, i.e., the asymptotic plane waves are multiplied by  $(2\pi)^{-3/2}$ . In other terms, the transition amplitude is that corresponding to the scattering of an electron, with initial momentum  $\mathbf{k}$  and final momentum  $\mathbf{k}'$ , by the KS potential  $V$ .

For small  $v$ , the integration in (11) can be simplified. First of all, we have to note that the integral of (11) over the unshifted Fermi sphere is zero since:

$$J = \int d\hat{\mathbf{k}} \int d\hat{\mathbf{k}}' [\hat{\mathbf{v}} \cdot (\hat{\mathbf{k}} - \hat{\mathbf{k}}')] |f(\mathbf{k}, \hat{\mathbf{k}}')|^2 \quad (13)$$

is zero along Lemma 1. This is also the case whenever the integration over  $\cos \theta_k$  runs from -1 to +1. Therefore, the integration over  $\mathbf{k}$  in (11) can be restricted to the volume of the shifted Fermi sphere outside the sphere of radius  $k - v$  (see Figure 1). Then, for a given orientation of  $\mathbf{k}$ , the lower bound on  $k$  is always  $k_F - v$ . The upper bound,  $k_m$ , is such that  $k_F = |\mathbf{k}_m + \mathbf{v}|$  which yields to first order in  $v$ :

$$k_m = k_F - v \cos \theta_k + 0(v) \quad (14)$$

and thus:

$$\int^{\text{SFS}} g(\mathbf{k}) d\mathbf{k} = \int d\hat{\mathbf{k}} \int_{k_F-v}^{k_F-v \cos \theta_k} k^2 g(\mathbf{k}) dk = \int d\hat{\mathbf{k}}_F k_F^2 g(\mathbf{k}_F) v (1 - \cos \theta_k) + 0(v) \quad (15)$$

Using the latter result in (11):

$$\frac{dE}{dZ} = \frac{k_F^4 v}{4\pi^3} \int d\hat{\mathbf{k}}_F \int d\hat{\mathbf{k}}'_F (1 - \hat{\mathbf{v}} \cdot \hat{\mathbf{k}}_F) [\hat{\mathbf{v}} \cdot (\hat{\mathbf{k}}_F - \hat{\mathbf{k}}'_F)] |f(\mathbf{k}_F, \hat{\mathbf{k}}'_F)|^2 \quad (16)$$

In (16), only the term  $\hat{\mathbf{v}} \cdot \hat{\mathbf{k}}$  from  $(1 - \hat{\mathbf{v}} \cdot \hat{\mathbf{k}})$  gives a non zero contribution along Lemma 1. Putting everything together, to first order in  $v$ , we end with the expression of the friction coefficient:

$$\Gamma_{\text{SFS}} = 4\pi k_F^4 \int d\hat{\mathbf{k}}_F \int d\hat{\mathbf{k}}'_F \hat{\mathbf{v}} \cdot \hat{\mathbf{k}}_F [\hat{\mathbf{v}} \cdot (\hat{\mathbf{k}}_F - \hat{\mathbf{k}}'_F)] \left| \int d\mathbf{r} [\phi_{\mathbf{k}'_F}(\mathbf{r})]^* V(\mathbf{r}) \Psi_{\mathbf{k}_F}^+(\mathbf{r}) \right|^2 \quad (17)$$

Let  $V_0$  be the KS potential for the static problem ( $v=0$ ). The usual procedure [2], to determine the energy loss, consists in using  $V_0$  in (17) instead of  $V$  and in replacing  $\Psi_{\mathbf{k}}^+(\mathbf{r})$  by the static KS orbital  $\psi_{\mathbf{k}}^+(\mathbf{r})$  (i.e., orbitals associated with  $V_0$ ). Let us prove that this procedure gives correctly the first order energy loss with respect to  $v$ . To this end, we make use of the distorted-wave theory, using  $V_0$  as a distortion potential.

In the distorted wave theory, the exact transition amplitude (1) for elastic scattering by  $V$  can be written as the sum of two terms. One is the transition amplitude under the action of the distortion potential alone:

$$f_{DW}^I(\mathbf{k}, \hat{\mathbf{k}}') = (2\pi)^2 \int d\mathbf{r} [\phi_{\mathbf{k}'}(\mathbf{r})]^* V_0(r) \psi_{\mathbf{k}}^+(\mathbf{r}) \quad (18)$$

i.e., the transition amplitude for the static problem. It corresponds to the expression usually calculated to obtain the energy loss [2, 3]. The other term is given by:

$$f_{DW}^{II}(\mathbf{k}, \hat{\mathbf{k}}') = (2\pi)^2 \int d\mathbf{r} [\psi_{\mathbf{k}'}^-(\mathbf{r})]^* [V(\mathbf{r}) - V_0(r)] \Psi_{\mathbf{k}}^+(\mathbf{r}) \quad (19)$$

The perturbation potential in (19) is no longer the full potential  $V(\mathbf{r})$  but only  $\Delta V = V - V_0$ , the difference between the KS potential for the moving atom and that for the atom at rest. The difference potential  $\Delta V$  is of order  $v$ , at least. Calculation of  $f_{DW}^{II}$  to first order in  $v$  corresponds to the first order of perturbation theory when the perturbation is  $\Delta V$ :

$$f_{DWB}^{II}(\mathbf{k}, \hat{\mathbf{k}}') = (2\pi)^2 \int d\mathbf{r} [\psi_{\mathbf{k}'}^-(\mathbf{r})]^* \Delta V(\mathbf{r}) \psi_{\mathbf{k}}^+(\mathbf{r}) \quad (20)$$

The quantity  $|f_{DWB}^{II}|^2$  is of order  $v^2$  and therefore negligible. However the cross term  $(f^I)^* f^{II}$  integrated over the *unshifted* Fermi sphere *might* give a contribution of order  $v$ . The integration of this cross-term over  $\hat{\mathbf{k}}$  and  $\hat{\mathbf{k}}'$  involves the expression (see Eq. 11 and 12):

$$J = \int d\hat{\mathbf{k}} \int d\hat{\mathbf{k}}' [\hat{\mathbf{v}} \cdot (\hat{\mathbf{k}} - \hat{\mathbf{k}}')] [f_{DW}^I(\mathbf{k}, \hat{\mathbf{k}}')]^* f_{DWB}^{II}(\mathbf{k}, \hat{\mathbf{k}}') \quad (21)$$

which is zero along Lemma 1<sup>1</sup>. This completes the proof that (18) gives correctly the friction coefficient as the coefficient of the first order in  $v$  of the energy loss. Therefore, to first order in  $v$ , the final expression for  $\Gamma_{\text{SFS}}$  is:

$$\Gamma_{\text{SFS}} = 4\pi k_F^4 \int d\hat{\mathbf{k}}_F \int d\hat{\mathbf{k}}'_F \cos\theta_{k_F} [\hat{\mathbf{v}} \cdot (\hat{\mathbf{k}}_F - \hat{\mathbf{k}}'_F)] \left| \int d\mathbf{r} [\phi_{\mathbf{k}'_F}(\mathbf{r})]^* V_0(\mathbf{r}) \psi_{\mathbf{k}_F}^+(\mathbf{r}) \right|^2 \quad (22)$$

### 3 Friction coefficient from HP

Consider now expression (12) of HP (to be consistent with our definition of  $\Gamma_{\text{SFS}}$ , we calculate  $M\Gamma_{\text{HP}}$ ). It reads:

$$\Gamma_{\text{HP}} = 2\pi \int d\mathbf{k} \int d\mathbf{k}' \left| \int d\mathbf{r} [\psi_{\mathbf{k}'}^-(\mathbf{r})]^* \frac{dV_0}{dQ} \psi_{\mathbf{k}}^+(\mathbf{r}) \right|^2 \delta(\epsilon_F - \epsilon_k) \delta(\epsilon_F - \epsilon_{k'}) \quad (23)$$

Using:

$$\int_0^\infty k^2 f(k) \delta(\epsilon_F - \epsilon_k) dk = \int_0^\infty \sqrt{2\epsilon_k} f(\sqrt{2\epsilon_k}) \delta(\epsilon_F - \epsilon_k) d\epsilon_k = k_F f(k_F) \quad (24)$$

$$\Gamma_{\text{HP}} = 2\pi k_F^2 \int d\hat{\mathbf{k}}_F \int d\hat{\mathbf{k}}'_F \left| \int d\mathbf{r} [\psi_{\mathbf{k}'_F}^-(\mathbf{r})]^* \frac{dV_0}{dQ} \psi_{\mathbf{k}_F}^+(\mathbf{r}) \right|^2 \quad (25)$$

The relation between the latter expression and (22) is not obvious. HP make use of two approximations in their derivation. The first one is the adiabatic approximation. This corresponds to the limit  $v \rightarrow 0$  and therefore their final expression should have, in this respect, the same status as (22). Furthermore, their calculation is based on linear theory (see the appendix of [1]), which should be equivalent to the use of perturbation theory, which is also used, as we have shown above, in the derivation of (22).

The difference between (22) and (25) lies in:

- (i) the presence of  $\psi_{\mathbf{k}'}^-$  instead of  $\phi_{\mathbf{k}'}$ .

---

<sup>1</sup>Note that in [4] the authors invoke the Born approximation to prove this property (see discussion following Eq. A2). As shown above, this is an exact property and perturbation theory is not required

(ii) the presence of  $dV_0/dQ$  instead of  $V_0$ , where  $dV_0/dQ$  is the derivative with respect to the impurity position.

(iii) the absence of the angular terms:  $\cos \theta_k [\hat{\mathbf{v}} \cdot (\hat{\mathbf{k}} - \hat{\mathbf{k}}')]$ .

So we are left with the question: is (25) equivalent to (22)?

## 4 Perturbation theory

It corresponds to the case of a vanishingly small potential  $V$  or  $V_0$ . Then, the amplitude (18) may be calculated in Born approximation:

$$\begin{aligned} f_B(\mathbf{k}, \hat{\mathbf{k}}') &= (2\pi)^2 \int d\mathbf{r} [\phi_{\mathbf{k}'}(\mathbf{r})]^* V_0(\mathbf{r}) \phi_{\mathbf{k}}(\mathbf{r}) \\ &= (2\pi)^2 (2\pi)^{-3} \int d\mathbf{r} e^{-i\mathbf{k}' \cdot \mathbf{r}} V_0(\mathbf{r}) e^{i\mathbf{k} \cdot \mathbf{r}} \\ &= (2\pi)^2 \tilde{V}_0(\mathbf{k} - \mathbf{k}') \end{aligned} \quad (26)$$

and the Born approximation to (22) is:

$$\Gamma_{\text{SFS}}^B = 4\pi k_F^4 \int d\hat{\mathbf{k}}_F \int d\hat{\mathbf{k}}'_F \cos \theta_{k_F} [\hat{\mathbf{v}} \cdot (\hat{\mathbf{k}}_F - \hat{\mathbf{k}}'_F)] |\tilde{V}_0(\mathbf{k}_F - \mathbf{k}'_F)|^2 \quad (27)$$

Similarly, the perturbation approximation to the  $\mathbf{r}$  integral in (25) gives:

$$(2\pi)^{-3} \int d\mathbf{r} e^{-i\mathbf{k}' \cdot \mathbf{r}} \frac{dV_0}{d(\hat{\mathbf{v}} \cdot \mathbf{r})} e^{i\mathbf{k} \cdot \mathbf{r}} = -i \hat{\mathbf{v}} \cdot (\mathbf{k} - \mathbf{k}') \tilde{V}_0(\mathbf{k} - \mathbf{k}') \quad (28)$$

We may use:

$$[\hat{\mathbf{v}} \cdot (\hat{\mathbf{k}} - \hat{\mathbf{k}}')]^2 = (\hat{\mathbf{v}} \cdot \hat{\mathbf{k}}')^2 - (\hat{\mathbf{v}} \cdot \hat{\mathbf{k}})^2 + 2(\hat{\mathbf{v}} \cdot \hat{\mathbf{k}}) [\hat{\mathbf{v}} \cdot (\hat{\mathbf{k}} - \hat{\mathbf{k}}')] \quad (29)$$

and note that:

$$\int d\hat{\mathbf{k}} \int d\hat{\mathbf{k}}' (\hat{\mathbf{v}} \cdot \hat{\mathbf{k}}')^2 |\tilde{V}_0(\mathbf{k} - \mathbf{k}')|^2 = \int d\hat{\mathbf{k}} \int d\hat{\mathbf{k}}' (\hat{\mathbf{v}} \cdot \hat{\mathbf{k}})^2 |\tilde{V}_0(\mathbf{k}' - \mathbf{k})|^2 \quad (30)$$

$$= \int d\hat{\mathbf{k}} \int d\hat{\mathbf{k}}' (\hat{\mathbf{v}} \cdot \hat{\mathbf{k}})^2 |\tilde{V}_0(\mathbf{k} - \mathbf{k}')|^2 \quad (31)$$

the last step following the transformation  $\hat{\mathbf{k}} \rightarrow -\hat{\mathbf{k}}$  and  $\hat{\mathbf{k}}' \rightarrow -\hat{\mathbf{k}}'$ . Therefore, we are left with:

$$\Gamma_{\text{HP}}^B = 4\pi k_F^4 \int d\hat{\mathbf{k}}_F \int d\hat{\mathbf{k}}'_F (\hat{\mathbf{v}} \cdot \hat{\mathbf{k}}_F) [\hat{\mathbf{v}} \cdot (\hat{\mathbf{k}}_F - \hat{\mathbf{k}}'_F)] |\tilde{V}_0(\mathbf{k}_F - \mathbf{k}'_F)|^2 \quad (32)$$

which is identical to (27). This is an indication that there is some relation between the expression of HP and that of the SFS.

## 5 Equivalence between both expressions of the friction coefficient

The preceding derivation puts us on the track of the solution. We introduce the potential  $V_1$  obtained by shifting the potential  $V_0$  by a small distance  $\delta Q$  along the direction of the velocity  $\hat{v}$ .

$$\lim_{\delta Q \rightarrow 0} V_1 = V_0 + \frac{dV_0}{dQ} \delta Q = V_0 + \delta V \quad (33)$$

In the following equations, we omit  $\lim_{\delta Q \rightarrow 0}$  for brevity.

### 5.1 Another Lemma

Let  $T(\delta Q \hat{v})$  be the translation operator for translation of  $\delta Q$  along the velocity. Its explicit form is given by, e.g., Cohen-Tannoudji *et al.*[5] in Eq. (19) of section I-EII:

$$T(\delta Q \hat{v}) = e^{i \delta Q \hat{v} \cdot \mathbf{P}} \quad (34)$$

where  $\mathbf{P}$  is the momentum operator. The action of the translation operator on a scattering function is simple when scattering takes place against a “background” with translation symmetry. This is the case in vacuum or in a jellium. This is *not* the case within a solid and the following discussion is not valid in the latter case.

Let  $\Xi_{\mathbf{k}}^+$  or  $\Xi_{\mathbf{k}}^-$  be any scattering wave function. In the case of a “background” with translation symmetry:

$$T(\delta Q \hat{v}) \Xi_{\mathbf{k}}^\pm = e^{i \delta Q \hat{v} \cdot \mathbf{k}} \Xi_{\mathbf{k}}^\pm = [1 + i \delta Q \hat{v} \cdot \mathbf{k} + 0(\delta Q^2)] \Xi_{\mathbf{k}}^\pm \quad (35)$$

As a consequence:

$$\begin{aligned} \langle \Xi_{\mathbf{k}'}^\pm | \delta V | \Xi_{\mathbf{k}}^\pm \rangle &= \langle \Xi_{\mathbf{k}'}^\pm | T^\dagger V_0 T - V_0 | \Xi_{\mathbf{k}}^\pm \rangle \\ &= \langle T \Xi_{\mathbf{k}'}^\pm | V_0 | T \Xi_{\mathbf{k}}^\pm \rangle - \langle \Xi_{\mathbf{k}'}^\pm | V_0 | \Xi_{\mathbf{k}}^\pm \rangle \\ &= i \delta Q \hat{v} \cdot (\mathbf{k} - \mathbf{k}') \langle \Xi_{\mathbf{k}'}^\pm | V_0 | \Xi_{\mathbf{k}}^\pm \rangle + 0(\delta Q^2) \end{aligned} \quad (36)$$

### 5.2 Transformation of HP expression (25)

We first show that (25) is equivalent, to first order in  $v$ , to the transition amplitude for scattering by the potential  $V_1$ :

$$g(\mathbf{k}, \hat{\mathbf{k}}') = (2\pi)^2 \langle \phi_{\mathbf{k}'} | V_1 | \Phi_{\mathbf{k}}^+ \rangle \quad (37)$$

where  $\Phi_{\mathbf{k}}^+$  is the wave function for scattering in the presence of  $V_1$ . To this end, we use the distorted-wave theory, with  $V_0$  as distorting potential, to evaluate (37)

$$g(\mathbf{k}, \hat{\mathbf{k}}') = (2\pi)^2 [\langle \phi_{\mathbf{k}'} | V_0 | \psi_{\mathbf{k}}^+ \rangle + \langle \psi_{\mathbf{k}'}^- | \delta V | \Phi_{\mathbf{k}}^+ \rangle] = g^I(\mathbf{k}, \hat{\mathbf{k}}') + g^{II}(\mathbf{k}, \hat{\mathbf{k}}') + 0(\delta Q^2) \quad (38)$$

We now integrate over  $\hat{\mathbf{k}}$  and  $\hat{\mathbf{k}}'$  as in (25). The integral of  $|g^I|^2$  is zero according to Lemma 2. To calculate the cross-term  $(g^I)^* g^{II}$  we use (36) for  $g^{II}$ . The result is zero according to Lemma

1. We are left with the term in  $|g^{II}|^2$ . Then,  $g^{II}$  is calculated in the Born approximation (first order in  $\delta Q$ ), i.e.,  $\Phi_{\mathbf{k}}^+$  is replaced by  $\psi_{\mathbf{k}}^+$ ,

$$K = \int d\hat{\mathbf{k}} \int d\hat{\mathbf{k}}' |g(\mathbf{k}, \hat{\mathbf{k}}')|^2 = (2\pi)^2 \int d\hat{\mathbf{k}} \int d\hat{\mathbf{k}}' \left| \int d\mathbf{r} [\psi_{\hat{\mathbf{k}}'}^-(\mathbf{r})]^* \frac{dV_0}{dQ} \delta Q \psi_{\mathbf{k}}^+(\mathbf{r}) \right|^2 \quad (39)$$

which contains the same matrix element as in (25). As a conclusion,

$$\Gamma_{\text{HP}} = 2\pi k_F^2 \int d\hat{\mathbf{k}}_F \int d\hat{\mathbf{k}}'_F \left| \int d\mathbf{r} [\phi_{\mathbf{k}'_F}(\mathbf{r})]^* \frac{V_1(\mathbf{r})}{\delta Q} \Phi_{\mathbf{k}_F}^+(\mathbf{r}) \right|^2 + 0(\delta Q^2) \quad (40)$$

On the other hand, (37) can be transformed by using (36):

$$g(\mathbf{k}, \hat{\mathbf{k}}') = (2\pi)^2 \left\{ \langle \phi_{\mathbf{k}'} | V_0 | \Phi_{\mathbf{k}}^+ \rangle + i \delta Q \hat{\mathbf{v}} \cdot (\mathbf{k} - \mathbf{k}') \langle \phi_{\mathbf{k}'} | V_0 | \Phi_{\mathbf{k}}^+ \rangle \right\} + 0(\delta Q^2) \quad (41)$$

To first order in  $\delta Q$ ,  $\Phi_{\mathbf{k}}^+ \rightarrow \psi_{\mathbf{k}}^+$ . Then:

$$g(\mathbf{k}, \hat{\mathbf{k}}') = (2\pi)^2 \left\{ \langle \phi_{\mathbf{k}'} | V_0 | \Phi_{\mathbf{k}}^+ \rangle + i \delta Q \hat{\mathbf{v}} \cdot (\mathbf{k} - \mathbf{k}') \langle \phi_{\mathbf{k}'} | V_0 | \psi_{\mathbf{k}}^+ \rangle \right\} + 0(\delta Q^2) = g^\alpha + g^\beta \quad (42)$$

Using again Lemma 2 for the integral of  $|g^\alpha|^2$  and Lemma 1 for that of the cross-term  $(g^\alpha)^* g^\beta$ , one gets:

$$K = \int d\hat{\mathbf{k}} \int d\hat{\mathbf{k}}' \left| \hat{\mathbf{v}} \cdot (\mathbf{k} - \mathbf{k}') \langle \phi_{\mathbf{k}'} | V_0 | \psi_{\mathbf{k}}^+ \rangle \right|^2 \quad (43)$$

A derivation identical to the one leading to (32) gives the final result:

$$K = 2k^2 \int d\hat{\mathbf{k}} \int d\hat{\mathbf{k}}' \hat{\mathbf{v}} \cdot \hat{\mathbf{k}} \left[ \hat{\mathbf{v}} \cdot (\hat{\mathbf{k}} - \hat{\mathbf{k}}') \right] \left| \langle \phi_{\mathbf{k}'} | V_0 | \psi_{\mathbf{k}}^+ \rangle \right|^2 \quad (44)$$

which proves the equivalence of (22) and (25) to first order in  $v$ .

It should be stressed that this equivalence is only verified when the “background” electronic density has translation symmetry. If not, as we have already noted, the simple transformation (35) of the scattering functions under a translation is not correct and, in addition, most of the expressions derived from scattering theory should be modified.

## References

- [1] B. Hellsing and M. Persson, Phys. Scripta **29**, 360 (1984).
- [2] E. Zaremba, A. Arnau, and P. M. Echenique, Nucl. Instrum. Methods B **96**, 619 (1995).
- [3] P. M. Echenique and M. E. Uranga, *Interaction of charged particles with solids and surfaces*, edited by A. Gras-Marti *et al.*, Plenum, New-York, 1991
- [4] A. Salin, A. Arnau, P. M. Echenique, and E. Zaremba, Phys. Rev. B **59**, 2537 (1999).
- [5] C. Cohen-Tannoudji, B. Diu, and F. Laloë, *Quantum mechanics* (Wiley-Interscience, New-York, 1977)

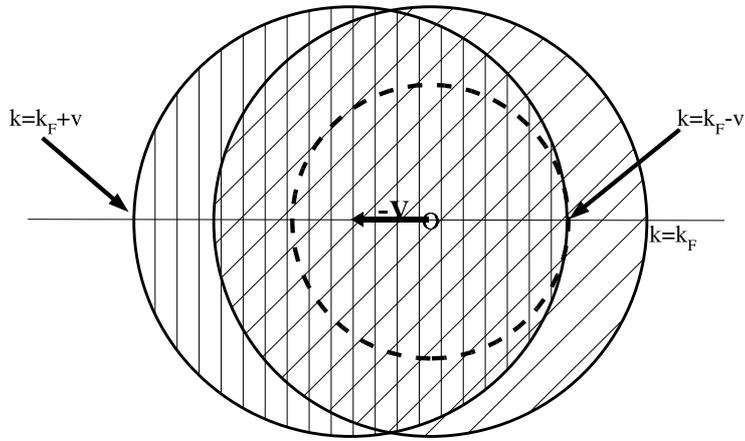

Figure 1: Schematic representation of the integration volume over  $\mathbf{k}$  in the shifted Fermi sphere. The cut through the original Fermi sphere ( $v = 0$ ) is given by the circle filled with a diagonal pattern and origin  $O$ . When  $v \neq 0$  the integration is performed over the Fermi sphere, shifted by  $-\mathbf{v}$ , filled with a vertical pattern. The added volume (with only vertical pattern) corresponds to  $k$  values larger than  $k_F$ . The subtracted volume (with only diagonal pattern) corresponds to  $k$  values smaller than  $k_F$ . This asymmetry is the cause of an energy transfer from the ion to the electrons. The dashed circle corresponds to the sphere of radius  $k_F - v$ .
