# Supplementary material for: Electronic friction for a slow impurity in an inhomogeneous metallic system
Source: arXiv:1302.0986 ancillary file (2013-02-05)
Supplement: Supplementary file 2 [file 2013.02.02_Note2.pdf]

## Note 2

A 1D model for friction in an inhomogenous jellium.

A. Salin<sup>1</sup>,

12, rue Jules Testaud, 33700 Mérignac, France

February 4, 2013

<sup>1</sup>Retired from Université de Bordeaux I

# Chapter 1

## 1D scattering for an asymptotically asymmetric potential

### 1.1 Definitions

We consider a one dimensional problem. The associated coordinate is  $z$ . The potential  $V(z)$  in which the particle moves goes to zero as  $z$  goes to  $+\infty$  and to a finite negative value when  $z$  goes to  $-\infty$ .

$$\lim_{z \rightarrow -\infty} V(z) = \Delta E = -|\Delta E| \quad (1.1)$$

We use throughout atomic units and assume, for simplicity, that the particle mass is 1.

#### 1.1.1 Positive energies

Let  $E$  be a given value of the energy ( $E > 0$ ). We define the momenta  $k_1$  and  $k_2$  through:

$$E = k_2^2/2 \quad (1.2a)$$

$$= k_1^2/2 + \Delta E \quad (1.2b)$$

i.e.,  $k_2$  (resp.  $k_1$ ) is the momentum associated with free motion at  $+\infty$  (resp.  $-\infty$ ) and  $k_1 > k_2$ . We introduce the wave functions  $B(z)$  and  $A(z)$  corresponding to ingoing (from  $+\infty$ ) and outgoing (from  $-\infty$ ) boundary conditions. They take asymptotically the following forms:

$$B(z) \xrightarrow{z \rightarrow +\infty} b' e^{ik_2 z} + b e^{-ik_2 z} \quad (1.3a)$$

$$\xrightarrow{z \rightarrow -\infty} \tilde{b} e^{-ik_1 z} \quad (1.3b)$$

$$A(z) \xrightarrow{z \rightarrow +\infty} \tilde{a} e^{ik_2 z} \quad (1.3c)$$

$$\xrightarrow{z \rightarrow -\infty} a' e^{-ik_1 z} + a e^{ik_1 z} \quad (1.3d)$$

Our notations are close to those of [1], chap. NIII. We normalize the incident flux on the  $\mathbf{k}$ -scale, so that:

$$a = b = 1/\sqrt{2\pi} \quad (1.4)$$

## 1.1.2 Negative energies

For negative energies, we impose that our solution decays exponentially for  $z$  going to  $+\infty$ .

$$A(z) \xrightarrow{z \rightarrow +\infty} \tilde{a} e^{-\alpha z} \quad (1.5a)$$

$$\xrightarrow{z \rightarrow -\infty} c \sin(k_1 z + \gamma_{k_1}) \quad (1.5b)$$

where  $\alpha = \sqrt{-2E}$  and  $c$  is a constant. Normalization on the  $\mathbf{k}$ -scale leads to the value  $c = 1/\sqrt{\pi}$ . Note also that the function is the same for  $\mathbf{k}_1$  and  $-\mathbf{k}_1$  ( $k_1 = |\mathbf{k}_1|$ ).

## 1.2 Determination of the wave functions

### 1.2.1 Positive energies

We introduce the new function:

$$\mathcal{B}(z) \xrightarrow{z \rightarrow +\infty} \beta' e^{ik_2 z} + \beta e^{-ik_2 z} \quad (1.6a)$$

$$\xrightarrow{z \rightarrow -\infty} e^{-ik_1 z} \quad (1.6b)$$

If  $\beta = \beta_r + i\beta_i$  and  $\beta' = \beta'_r + i\beta'_i$ ,

$$\begin{aligned} \lim_{z \rightarrow +\infty} \mathcal{B}(z) &= (\beta_r + \beta'_r) \cos(k_2 z) + (\beta_i - \beta'_i) \sin(k_2 z) \\ &\quad + i(\beta_i + \beta'_i) \cos(k_2 z) + i(\beta'_r - \beta_r) \sin(k_2 z) \end{aligned} \quad (1.7)$$

We integrate the Schrödinger equation from a large negative  $z$  to determine the real functions  $\mathcal{B}_1$  and  $\mathcal{B}_2$  behaving respectively as  $\cos(k_1 z)$  and  $\sin(k_1 z)$  in this limit. Then,  $\mathcal{B}(z) = \mathcal{B}_1(z) - i\mathcal{B}_2(z)$ . This allows us to determine  $\beta$  and  $\beta'$  by identification with expression (1.7) at two different values of  $z$ , say  $z_a$  and  $z_b$ , in the large  $z$  region where the potential is zero. If  $\text{cosa} = \cos(k_2 z_a)$ ,  $\text{cosb} = \cos(k_2 z_b)$ ,  $\text{sina} = \sin(k_2 z_a)$ ,  $\text{sinb} = \sin(k_2 z_b)$ ,  $\mathcal{B}_{1,2}^{a,b} = \mathcal{B}_{1,2}(z_{a,b})$ , then:

$$2\beta_r(\text{cosa sinb} - \text{sina cosb}) = \mathcal{B}_1^a \text{sinb} - \mathcal{B}_1^b \text{sina} - \mathcal{B}_2^a \text{cosb} + \mathcal{B}_2^b \text{cosa} \quad (1.8a)$$

$$2\beta'_r(\text{cosa sinb} - \text{sina cosb}) = \mathcal{B}_1^a \text{sinb} - \mathcal{B}_1^b \text{sina} + \mathcal{B}_2^a \text{cosb} - \mathcal{B}_2^b \text{cosa} \quad (1.8b)$$

$$2\beta_i(\text{cosa sinb} - \text{sina cosb}) = -\mathcal{B}_1^a \text{cosb} + \mathcal{B}_1^b \text{cosa} - \mathcal{B}_2^a \text{sinb} + \mathcal{B}_2^b \text{sina} \quad (1.8c)$$

$$2\beta'_i(\text{cosa sinb} - \text{sina cosb}) = \mathcal{B}_1^a \text{cosb} - \mathcal{B}_1^b \text{cosa} - \mathcal{B}_2^a \text{sinb} + \mathcal{B}_2^b \text{sina} \quad (1.8d)$$

An important property of the wave function is current conservation. The current at  $z$ ,  $J(z)$ , associated with  $B(z)$  is given by:

$$J(z) = \left( B(z)^* \frac{d}{dz} B(z) - B(z) \frac{d}{dz} B(z)^* \right) / 2i \quad (1.9)$$

Applying (1.9) at  $+\infty$  and  $-\infty$ , one gets:

$$|\beta|^2 - |\beta'|^2 = k_1/k_2 \quad (1.10)$$

Once  $\mathcal{B}$  is known, we obtain  $B(z)$  through the relation:

$$B(z) = \mathcal{B}(z) / \beta \sqrt{2\pi} \quad (1.11)$$

and therefore:

$$b' = \beta'/\beta\sqrt{2\pi} \quad (1.12a)$$

$$\tilde{b} = 1/\beta\sqrt{2\pi} \quad (1.12b)$$

The reflection probability,  $P_r$ , and the transmission probability,  $P_t$ , are given by:

$$P_r = |b'/b|^2 = |\beta'/\beta|^2 \quad (1.13a)$$

$$P_t = |\tilde{b}/b|^2 k_1/k_2 = k_1/|\beta|^2 k_2 \quad (1.13b)$$

The factor  $k_1/k_2$  in the latter expression arises from the fact that the particles are accelerated in the large negative  $z$  region with respect to the large positive  $z$  region by the factor  $k_1/k_2$ . We can observe that the conservation of current (1.10) is then equivalent to  $P_t = 1 - P_r$  as it should.

We now set to determine the function  $A(z)$ . We could, of course, follow a procedure similar to that used in the determination of  $B(z)$ , i.e., introduce the new function:

$$\mathcal{A}(z) \xrightarrow{z \rightarrow +\infty} e^{ik_2 z} \quad (1.14a)$$

$$\xrightarrow{z \rightarrow -\infty} \alpha' e^{-ik_1 z} + \alpha e^{ik_1 z} \quad (1.14b)$$

Integrating the Schrödinger equation from a large positive  $z$ , we may determine the real functions  $\mathcal{A}_1$  and  $\mathcal{A}_2$  behaving respectively as  $\cos(k_2 z)$  and  $\sin(k_2 z)$  in this limit and  $\mathcal{A}(z) = \mathcal{A}_1(z) + i\mathcal{A}_2(z)$ . This allows us to determine  $\alpha$  and  $\alpha'$  by identification with (1.14b) for large negative  $z$ . However, this is not necessary. As the Hamiltonian is real, the functions  $\mathcal{B}(z)$  and  $\mathcal{B}^*(z)$  are independent solutions of the Schrödinger equation. Consequently:

$$\mathcal{A}(z) = \zeta \mathcal{B}(z) + \xi \mathcal{B}^*(z) \quad (1.15)$$

Using (1.6) and (1.15) for  $z \rightarrow -\infty$ , one immediately gets  $\alpha = \xi$  and  $\alpha' = \zeta$ . On the other hand, in the limit  $z \rightarrow +\infty$  we obtain the system of equations:

$$\zeta \beta' + \xi \beta^* = 1 \quad (1.16a)$$

$$\zeta \beta + \xi (\beta')^* = 0 \quad (1.16b)$$

and finally, using (1.10):

$$\alpha = \beta k_2/k_1 \quad (1.17a)$$

$$\alpha' = -(\beta')^* k_2/k_1 \quad (1.17b)$$

Current conservation yields the relation:

$$|\alpha|^2 - |\alpha'|^2 = k_2/k_1 \quad (1.18)$$

The reflection probability is given by an expression similar to (1.13):

$$P_r = |a'/a|^2 = |\alpha'/\alpha|^2 \quad (1.19a)$$

$$P_t = |\tilde{a}/a|^2 k_2/k_1 = k_2/|\alpha|^2 k_1 \quad (1.19b)$$

Using (1.17), we can check that the reflection and transmission probabilities are the same for the ingoing and outgoing solutions, in spite of the asymmetry in the potential. This is equivalent to microreversibility for the 3-dimensional case.

Finally, we obtain the relation between  $A$  and  $B$  functions through:

$$A(z) = -(\beta')^* B(z) + \beta^* B^*(z) \quad (1.20a)$$

$$B(z) = -(\alpha')^* A(z) + \alpha^* A^*(z) \quad (1.20b)$$

We have checked that our results are the same when the  $A$  function is determined directly or from the  $B$  function, which is a good check on the integration accuracy.

## 1.2.2 Negative energies

To determine the solution, we start the integration from  $+\infty$  and adjust the function to its asymptotic form at large negative  $z$ .

## 1.3 Integral expression for the reflexion amplitude

The Schrödinger equation for  $\mathcal{B}$  is:

$$\left[ -\frac{1}{2} \frac{d^2}{dz^2} + V(z) \right] \mathcal{B}(z) = \frac{1}{2} k_2^2 \mathcal{B}(z) \quad (1.21)$$

Accordingly:

$$I = \int_{-\infty}^{+\infty} dz \left[ e^{-ik_2 z} \frac{d^2}{dz^2} \mathcal{B}(z) - \mathcal{B}(z) \frac{d^2}{dz^2} e^{-ik_2 z} \right] = 2 \int_{-\infty}^{+\infty} dz e^{-ik_2 z} V(z) \mathcal{B}(z) \quad (1.22)$$

Integrating by parts the l.h.s.:

$$\begin{aligned} I = & \lim_{z \rightarrow \infty} \left[ e^{-ik_2 z} \frac{d}{dz} \mathcal{B}(z) - \mathcal{B}(z) \frac{d}{dz} e^{-ik_2 z} \right] \\ & - \lim_{z \rightarrow -\infty} \left[ e^{-ik_2 z} \frac{d}{dz} \mathcal{B}(z) - \mathcal{B}(z) \frac{d}{dz} e^{-ik_2 z} \right] \\ & - \int_{-\infty}^{+\infty} dz \left[ \frac{d}{dz} e^{-ik_2 z} \frac{d}{dz} \mathcal{B}(z) - \frac{d}{dz} \mathcal{B}(z) \frac{d}{dz} e^{-ik_2 z} \right] \end{aligned} \quad (1.23)$$

The last term is obviously zero. The first one yields  $2ik_2\beta'$  and the second one:

$$- \lim_{x \rightarrow -\infty} i(k_2 - k_1) e^{-i(k_1+k_2)z} \quad (1.24)$$

Assume that for  $z < z_0$  the potential has reached its asymptotic limit  $(k_2^2 - k_1^2)/2$ . After some trivial algebra the final result is:

$$\beta' = \frac{1}{ik_2} \left[ \int_{z_0}^{+\infty} dz e^{-ik_2 z} V(z) \mathcal{B}(z) + \frac{i}{2} (k_2 - k_1) e^{-i(k_1+k_2)z_0} \right] \quad (1.25)$$

We introduce the normalized plane wave  $\phi_k(z) = e^{ikz}/\sqrt{2\pi}$ . Then, the reflexion amplitude  $F_r = \beta'/\beta$  is:

$$F_r = \frac{2\pi}{ik_2} \left[ \int_{z_0}^{+\infty} dz \phi_{k_2}^*(z) V(z) \mathcal{B}(z) + \frac{i}{2} (k_2 - k_1) \frac{e^{-i(k_1+k_2)z_0}}{2\pi\beta} \right] \quad (1.26)$$

an expression which looks like that of the 3D case. Note that the second term on the r.h.s. is zero when the potential goes to zero at  $-\infty$  and, therefore, appears only because of the asymptotic asymmetry of the potential.

Similarly, one can derive the integral expression for the transmission amplitude:

$$F_t = -i\sqrt{\frac{2\pi}{k_1 k_2}} \left[ \int_{-\infty}^{z_0} dz \phi_{-k_1}^*(z) V'(z) B(z) + \frac{i}{2} \frac{\beta'}{\beta} \frac{(k_1 - k_2)}{2\pi} e^{i(k_1+k_2)z_0} + \frac{i}{2} \frac{(k_1 + k_2)}{2\pi} e^{i(k_1-k_2)z_0} \right] \quad (1.27)$$

where  $V'(z) = V(z) + (k_1^2 - k_2^2)/2$ .

### 1.3.1 Distorted-wave theory

We split the potential into two parts:

$$V(z) = V_0(z) + W(z) \quad ; \quad \lim_{|z| \rightarrow \infty} W(z) = 0 \quad (1.28)$$

where  $V_0$  is the distortion potential. Let  $\mathcal{A}_0$  and  $\mathcal{B}_0$  be the solutions of the Schrödinger equation in the presence of  $V_0$  alone. The asymptotic conditions are similar to (1.6) and (1.14):

$$\mathcal{B}_0(z) \xrightarrow{z \rightarrow +\infty} \beta'_0 e^{ik_2 z} + \beta_0 e^{-ik_2 z} \quad (1.29a)$$

$$\xrightarrow{z \rightarrow -\infty} e^{-ik_1 z} \quad (1.29b)$$

$$\mathcal{A}_0(z) \xrightarrow{z \rightarrow -\infty} \alpha_0 e^{ik_1 z} + \alpha'_0 e^{-ik_1 z} \quad (1.29c)$$

$$\xrightarrow{z \rightarrow +\infty} e^{ik_2 z} \quad (1.29d)$$

We proceed as in the previous section:

$$\mathcal{I} = \int_{-\infty}^{+\infty} dz \left[ \mathcal{A}_0(z) \frac{d^2}{dz^2} \mathcal{B}(z) - \mathcal{B}(z) \frac{d^2}{dz^2} \mathcal{A}_0(z) \right] = 2 \int_{-\infty}^{+\infty} dz \mathcal{A}_0(z) W(z) \mathcal{B}(z) \quad (1.30)$$

Integrating by parts the l.h.s:

$$\begin{aligned} \mathcal{I} &= \lim_{z \rightarrow \infty} \left[ \mathcal{A}_0(z) \frac{d}{dz} \mathcal{B}(z) - \mathcal{B}(z) \frac{d}{dz} \mathcal{A}_0(z) \right] \\ &- \lim_{z \rightarrow -\infty} \left[ \mathcal{A}_0(z) \frac{d}{dz} \mathcal{B}(z) - \mathcal{B}(z) \frac{d}{dz} \mathcal{A}_0(z) \right] \\ &- \int_{-\infty}^{+\infty} dz \left[ \frac{d}{dz} \mathcal{A}_0(z) \frac{d}{dz} \mathcal{B}(z) - \frac{d}{dz} \mathcal{B}(z) \frac{d}{dz} \mathcal{A}_0(z) \right] \end{aligned} \quad (1.31)$$

The last term is obviously zero. The first one yields  $-2ik_2\beta$  and the second one  $-2ik_1\alpha_0$ . Using (1.17),  $k_1\alpha_0 = k_2\beta_0$  so that:

$$-\beta - \beta_0 = \frac{1}{ik_2} \int_{-\infty}^{+\infty} dz \mathcal{A}_0(z) W(z) \mathcal{B}(z) \quad (1.32)$$

or using (1.12) and (1.13):

$$F_t = -F_t^0 + i\sqrt{\frac{2\pi}{k_1 k_2}} \int_{-\infty}^{+\infty} dz A_0(z) W(z) B(z) \quad (1.33)$$

The l.h.s. is the transmission amplitude for the full potential  $V(z)$ . On the r.h.s. the first term is the transmission amplitude for the potential  $V_0(z)$  alone. The last term involves the distorted wave-function  $A_0$  and describes the transmission by  $W$  in the presence of  $V_0$ .

Similarly, the expression for the reflexion amplitude is:

$$F_r = F_r^0 + \frac{2\pi}{ik_2} \int_{-\infty}^{+\infty} dz B_0(z) W(z) B(z) \quad (1.34)$$

# Chapter 2

## Impurity in a 1D jellium

Throughout this chapter we speak for convenience of “electrons” and “positive charges” though the particles we consider have no reality. We do this only to facilitate the intuitive correspondence with the usual three dimensional problem. We use atomic units but never mention any unit since this is immaterial for our model which has only a qualitative value. We use throughout a screened regularized coulomb potential to describe the interaction between two particles located at  $z$  and  $z'$  respectively:

$$v_c^\pm(z, z') = \pm e^{-\alpha|z-z'|}/[|z-z'| + \varepsilon] \quad (2.1)$$

### 2.1 Homogenous jellium

#### 2.1.1 Basic properties

We wish to solve the Schrödinger equation for the Kohn-Sham orbitals:

$$\left[ -\frac{1}{2} \frac{d^2}{dz^2} + v_{KS}(z) \right] \varphi_{\mathbf{k}}(z) = \epsilon_{\mathbf{k}} \varphi_{\mathbf{k}}(z) \quad (2.2)$$

when the electrons move in a uniform density,  $n_0^+$ , of positive charges. The Kohn-Sham potential,  $v_{KS}$ , includes three components:

- The interaction potential with the background of positive particles:

$$v_+(z) = \int_{-\infty}^{+\infty} dz' n_0^+ v_c^-(z, z') \quad (2.3)$$

where  $n_0^+$  is the density of background particles.

- The Hartree potential:

$$v_H(z) = \int_{-\infty}^{+\infty} dz' n(z') v_c^+(z, z') \quad (2.4)$$

- The exchange-correlation potential  $v_{xc}[n(z)]$ .

In the present situation,  $v_H + v_+ = 0$  so that the Kohn-Sham functions are solution of:

$$\left[ -\frac{1}{2} \frac{d^2}{dz^2} + v_{xc}(n) \right] \varphi_{\mathbf{k}}(z) = \epsilon_{\mathbf{k}} \varphi_{\mathbf{k}}(z) \quad (2.5)$$

as in the 3D case. We use the convention that  $\mathbf{k} \in [-\infty, +\infty]$  and  $k = |\mathbf{k}|$ . As a consequence,

$$\varphi_{\mathbf{k}}(z) = (2\pi)^{-1/2} e^{i\mathbf{k}z}, \quad (2.6)$$

if normalization is on the k-scale, and  $\epsilon_{\mathbf{k}} = k^2/2 + v_{xc}(n)$ . In the paramagnetic case, the Fermi momentum,  $k_F$ , is defined by the relation:

$$n = 2 \int_{-k_F}^{+k_F} d\mathbf{k} |\varphi_{\mathbf{k}}(z)|^2 = 2k_F/\pi \quad (2.7)$$

We introduce the Wigner-Seitz distance,  $z_s = 1/n$ , i.e. the distance containing one charge.

For completeness we evaluate the exchange energy for the Hartree-Fock case, though we won't use it in the following study. The interaction between particles is described by a regularized Coulomb potential,  $1/[|z - z'| + \varepsilon]$ , or a screened regularized Coulomb potential,  $e^{-\alpha|z-z'|}/[|z - z'| + \varepsilon]$ . Let  $e_x$  be the energy density due to the electron-electron interaction. The interaction energy at  $z$  is given by :

$$E_x = n e_x = \int_{-k_F}^{+k_F} d\mathbf{k} \int_{-k_F}^{+k_F} d\mathbf{k}' \int_{-\infty}^{+\infty} dz' \varphi_{\mathbf{k}}(z) \varphi_{\mathbf{k}}^*(z') \varphi_{\mathbf{k}'}^*(z) \varphi_{\mathbf{k}'}(z') [|z - z'| + \varepsilon]^{-1} \quad (2.8a)$$

$$= \int_{-\infty}^{+\infty} dz' [|z - z'| + \varepsilon]^{-1} |f(z, z')|^2 \quad (2.8b)$$

where  $f(z, z') = \sin[k_F(z - z')]/\pi(z - z')$ . Finally,

$$e_x = \frac{1}{\pi} k_F I(k_F \varepsilon) \quad (2.9)$$

with:

$$I(Z) = \int_0^{\infty} dy y^{-2} (y + Z)^{-1} \sin^2 y \quad (2.10)$$

and the exchange potential is given by:

$$v_x = e_x + n \frac{de_x}{dn} = 2e_x - \frac{\varepsilon}{\pi} k_F^2 I'(k_F \varepsilon) \quad (2.11)$$

$$I'(Z) = \int_0^{\infty} dy y^{-2} (y + Z)^{-2} \sin^2 y \quad (2.12)$$

For the spin polarized case, one obtains:

$$e_x^{\pm} = \frac{1}{\pi} k_F^{\pm} I(k_F^{\pm} \varepsilon) \quad (2.13)$$

and

$$v_x^{\pm} = e_x^{\pm} + n^{\pm} \frac{de_x^{\pm}}{dn^{\pm}} = 2e_x^{\pm} - \frac{\varepsilon}{\pi} (k_F^{\pm})^2 I'(k_F^{\pm} \varepsilon) \quad (2.14)$$

where  $k_f^{\pm} = \pi n^{\pm}$ .

For the case of an exponentially screened regularized coulomb potential, one has to add a factor  $\exp(-\alpha y/k_F)$  in the integrand of  $I$  and  $I'$ .

Results are given in Fig. 2.1

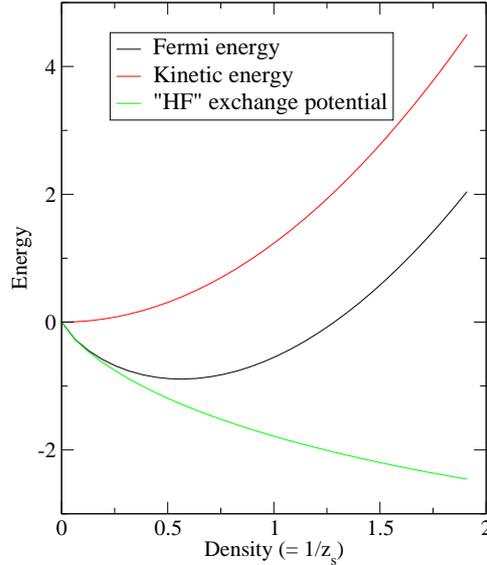

Figure 2.1: Fermi energy (w.r.t. band bottom) as a function of density. Red curve: kinetic energy  $k_F^2/2$ ; green curve: exchange potential obtained by using Kohn-Sham orbitals and the HF expression for the exchange energy.

### 2.1.2 Impurity in a homogenous linear jellium

We assume that the impurity is centered at  $z = 0$ . The interaction potential with the impurity is defined by:

$$v_{\text{imp}}(z) = v_c^-(z, 0) \quad (2.15)$$

In the following work we always use as parameters  $\alpha = 4$  and  $\varepsilon = 0.1$ . Then, the potential supports one bound singly occupied state with energy -1.275.

The problem at stake is independent of the model we are using. So, from now on we disregard the exchange-correlation potential. The screened regularized coulomb potential used to calculate the Hartree potential involves the parameters  $\alpha = 2$  and  $\varepsilon = 0.1$ . We solve the Kohn-Sham equation by an iterative procedure, as usual.

The determination of the density involves a sum over  $\mathbf{k}$ . Here, for a given energy, i.e., a given  $\mathbf{k}$ , the positive value of  $k$  is associated with a  $B$  function, here noted  $B_k$ , while negative values are associated with a  $A$  function, noted  $A_k$ . Then:

$$n(z) = m_b \sum_b |F_b(z)|^2 + 2 \int_0^{k_F} dk \left[ |A_k(z)|^2 + |B_k(z)|^2 \right] \quad (2.16)$$

where  $F_b$  is a bound Kohn-Sham orbital. The occupation of the bound states is defined by  $m_b$  which may take the values 0, 1 or 2 (remember that we don't consider the exchange-polarization potential in our calculations). The factor of 2 in front of the integral accounts for the two spin states.

Typical results, for  $m_b=2$ , are given in Fig. 2.2, where we have plotted the density in presence of the impurity divided by  $n_0^+$ . These results look qualitatively like those of the 3D case. The energy of the doubly occupied bound state is -0.410.

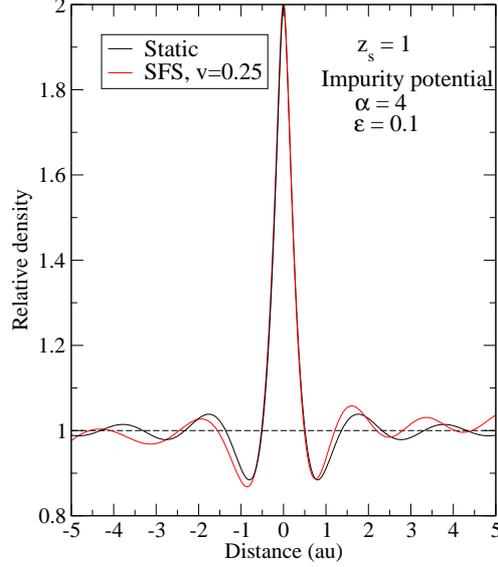

Figure 2.2: Density in the presence of an impurity divided by the density in absence of impurity for  $z_s = 1$  and a doubly occupied bound state.

### 2.1.3 Shifted Fermi Surface (SFS)

Note: we use the term Fermi surface in spite of the fact that in 1D it's not a surface!

The only difference with respect to the previous case is that the integration over  $\mathbf{k}$  now runs from  $-k_F + v$  to  $k_F + v$ , where  $v$  is the impurity velocity:

$$n_v(z) = m_b \sum_b |F_b(z)|^2 + 2 \int_0^{k_F - v} dk |A_k(z)|^2 + 2 \int_0^{k_F + v} dk |B_k(z)|^2 \quad (2.17)$$

Results are shown as the red curve in Fig. 2.2 for a velocity of 0.25 au. The backward-forward asymmetry is clearly visible in that figure. It is the origin of the stopping power.

### 2.1.4 Friction coefficient

For low velocities, as we show below, the stopping power varies linearly with impurity velocity. The coefficient of this linear term is the friction coefficient. We calculate this coefficient in two different ways.

#### From the SFS calculation

Let  $Z(t)$  be the position of the impurity at time  $t$  and  $\Psi(z; Z)$  the Kohn-Sham wave-function (a single Slater determinant of Kohn-Sham orbitals by definition) calculated for the SFS. The stopping power is given by:

$$\frac{d}{dZ} E(Z) = \frac{d}{dZ} \langle \Psi(z; Z) | H(Z) | \Psi(z; Z) \rangle \quad (2.18)$$

As the Kohn-Sham Hamiltonian is a one-particle operator and  $\Psi$  a single determinant:

$$\frac{d}{dZ} E(Z) = \int_{-\infty}^{+\infty} dz n_v(z) \left[ \frac{d}{dZ} \Big|_{Z=0} v_{\text{imp}}(z - Z) \right] \quad (2.19)$$

Table 2.1: Stopping power and friction coefficient for an impurity in a homogenous 1D jellium. The stopping power estimated from (2.19) as a function of velocity is fitted by  $a_0v + a_1v^2 + a_2v^3$ . Results on the last line are evaluated from (2.23b). Calculations are done for  $z \in [-5, 5]$  and  $\Delta z = 0.01$

| v                     | $z_s = 0.75$        | $z_s = 1.$          | $z_s = 1.5$         |
|-----------------------|---------------------|---------------------|---------------------|
| 0.01                  | 0.00472             | 0.00380             | 0.00235             |
| 0.02                  | 0.00947             | 0.00761             | 0.00470             |
| 0.03                  | 0.01425             | 0.01146             | 0.00710             |
| 0.04                  | 0.01908             | 0.01535             | 0.00953             |
| 0.05                  | 0.02398             | 0.01931             | 0.0120              |
| 0.06                  | 0.02897             | 0.02336             | 0.01456             |
| 0.07                  | 0.03406             | 0.0275              | 0.01719             |
| 0.08                  | 0.0393              | 0.0317              | 0.01992             |
| 0.09                  | 0.0446              | 0.0361              | 0.02274             |
| 0.1                   | 0.0501              | 0.0406              | 0.0257              |
| $\underline{a_0}$     | $\underline{0.471}$ | $\underline{0.379}$ | $\underline{0.234}$ |
| $a_1$                 | 0.034               | 0.0103              | 0.006               |
| $a_2$                 | 2.61                | 2.56                | 2.204               |
| Friction from (2.23b) | $\underline{0.474}$ | $\underline{0.373}$ | $\underline{0.239}$ |

and the friction coefficient is:

$$F = \lim_{v \rightarrow 0} \frac{1}{v} \int_{-\infty}^{+\infty} dz n_v(z) \left[ \frac{d}{dZ} \Big|_{Z=0} v_{\text{imp}}(z - Z) \right] \quad (2.20)$$

The stopping power is given in Table 2.1 for various velocities. We extract the coefficient of the term linear in  $v$  at low velocities by a polynomial least square fit. The latter value can be compared with the direct calculation of the friction coefficient as in the following subsection.

### Direct calculation of the friction coefficient

Here we assume that the mass  $\mu$  of the impurity is much larger than that of the electrons and calculate the energy loss to first order in their mass ratio.

Let an electron, with momentum  $\mathbf{k}$ , collide with the impurity, with momentum  $p$ . The projectile energy change when this electron is reflected is:

$$\Delta E = p^2/2\mu - (p - 2\mathbf{k})^2/2\mu = 2\mathbf{k}v + 0(1/\mu) \quad (2.21)$$

where  $v$  is the impurity velocity. The flux of incident particles being  $k/2\pi$ , the energy-loss per unit path length is given by:

$$\frac{dE}{dZ} = \frac{1}{v} \frac{dE}{dt} = \frac{2}{v} \int dk \left[ \frac{k}{2\pi} \right] [2\mathbf{k}v] P_r(k) \quad (2.22)$$

where  $P_r$  is the reflexion probability for a static impurity. The factor of 2 in front of the integral accounts for the two spin states. The fact that we may use the reflexion probability for a static

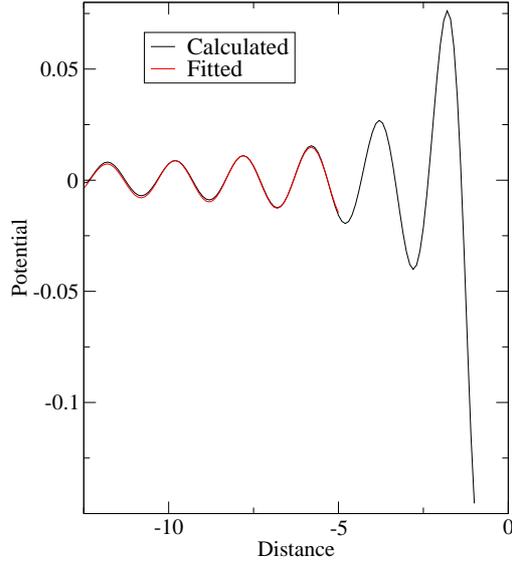

Figure 2.3: Behavior of the potential at large distances for  $z_s = 1$ . The impurity is the same as for Fig. 2.2. The red curve corresponds to a least square fit of the data for  $z < -5$ . The fitting curve is:  $-0.086 \sin(2k_F z + 1.01)/z$ .

impurity can be justified as for the 3D case. Then, in the SFS approach, the friction coefficient is:

$$F = \lim_{v \rightarrow 0} \frac{1}{v} \frac{dE}{dZ} = \lim_{v \rightarrow 0} \frac{2}{v\pi} \int_{-k_f+v}^{k_f+v} dk k^2 \text{sign}(k) P_r(k) \quad (2.23a)$$

$$= \frac{4}{\pi} k_F^2 P_r(k_F) + 0(v) \quad (2.23b)$$

The friction coefficient, as calculated by both methods, is shown in Table 2.1 for various values of  $z_s$ .

## Discussion

Results given in Table 2.1 are obtained by putting the problem into a *box* limited by  $z = -5$  and  $z = 5$ . This is necessary because results do not converge as the size of the box is enlarged. The reason is that the Hartree potential, far from the impurity, is proportional to  $\sin(2kz + \gamma)/z$ . This is illustrated in Fig. 2.3. Remember that the reflection probability is given by  $\beta'/\beta$  where  $\beta'$  as given by (1.25) contains the term:

$$\beta'_H = \frac{1}{ik} \int dz e^{-ikz} v_H(z) \mathcal{B}(z) \quad (2.24)$$

Let us study the behavior of this integral for large negative  $z$ . Then  $\mathcal{B}(z) = \exp(-ikz)$ . Therefore, the contribution from  $z_0$  to  $z_1$  (both large negative  $z$ ) is:

$$\delta\beta'_H \sim \int_{z_0}^{z_1} dz \frac{e^{-2ikz}}{z} [e^{2ikz+i\gamma} - e^{-2ikz-i\gamma}] \quad (2.25a)$$

$$\sim \ln(z_1/z_0) + 0(1/z) \quad (2.25b)$$

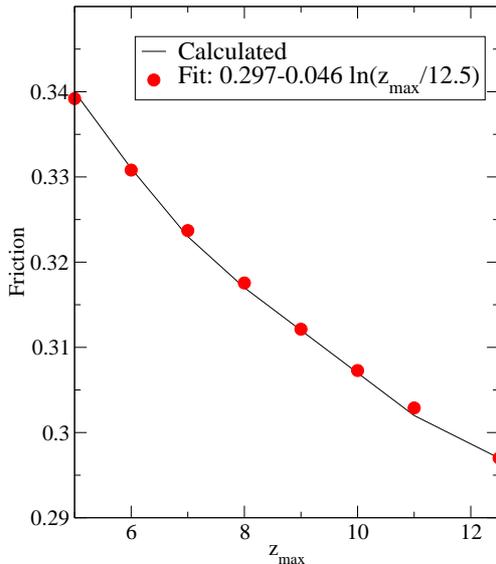

Figure 2.4: Friction coefficient. The potential used in the calculations is that of Fig. 2.3. The minimum  $z$  is kept equal to  $-12.5$ . Calculations are made for various values of the upper  $z$  limit,  $z_{\max}$ , and the results are fitted by a least square method.

This behavior is illustrated in Fig. 2.4. It is not a drawback for the problem we are interested in. In fact, there is no need to construct a “realistic” model and we may decide to study the case of a finite box. In addition, we have checked that the border effect is negligible: if we force the Hartree potential to go to zero in the vicinity of the box limit in various ways, the results do not change appreciably. What matters is the effective range in  $z$  because of the logarithmic divergence exhibited above.

## 2.2 Inhomogeneous jellium

### 2.2.1 Basic properties

We now consider an inhomogeneous jellium which is created by an external potential, referred to as the *step potential*, going to zero for  $z \rightarrow \infty$  and to a finite negative value,  $\Delta V$ , for  $z \rightarrow -\infty$ , as shown in Fig. 2.5. To be specific, we define this potential by:

$$v_{\text{step}}(z) = 0.5 \Delta V \{1 + \cos[\pi(z - z_1)/(z_2 - z_1)]\} \quad (z_1 < z < z_2) \quad (2.26a)$$

$$= \Delta V \quad (z < z_1) \quad (2.26b)$$

$$= 0 \quad (z > z_2) \quad (2.26c)$$

This potential has the required behavior at large  $|z|$  and a continuous derivative. The values of  $z_1$  and  $z_2$  determine the steepness of the slope between  $z_1$  and  $z_2$ . The value of  $\Delta V$  may be fixed by imposing a given value of  $z_s$  at large distances:  $z_s^1$  for  $z < 0$  and  $z_s^2$  for  $z > 0$ . Then,  $\Delta V = \epsilon_2^F - \epsilon_1^F$  where  $\epsilon_{1,2}^F = (k_{1,2}^F)^2/2$  (see Fig. 2.5). We may simulate a surface by imposing a large value for  $z_s^2$  which corresponds to a small value of the density at large positive  $z$ . For positive energies, a given value of  $k$  is associated with both an ingoing ( $B(z)$ ) and outgoing

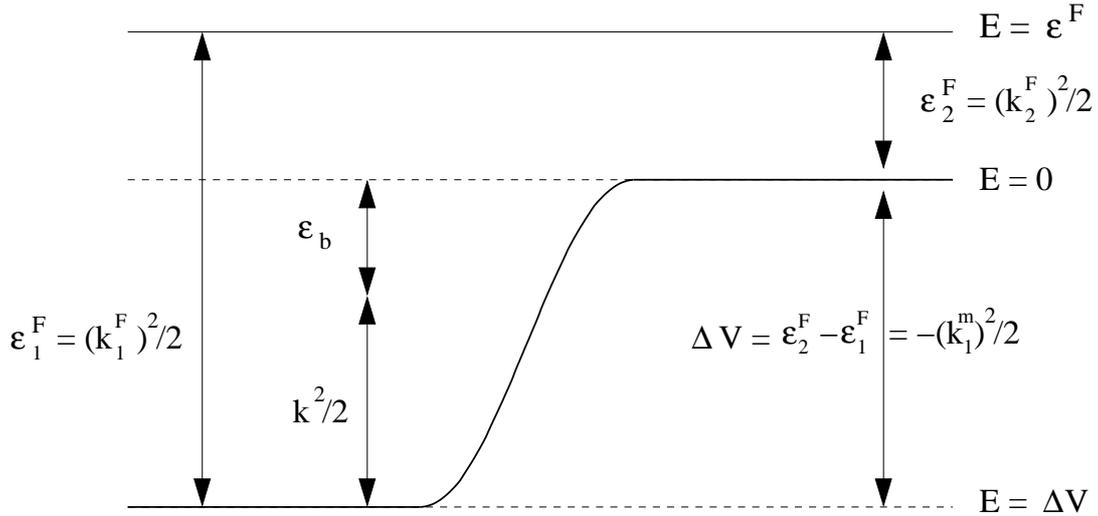

Figure 2.5: Sketch of the background potential used to define the inhomogeneous jellium.

( $A(z)$ ) wave-function. We label them here as  $B_2(k_2)$  and  $A_1(k_1)$ . For negative energies, we consider only those functions,  $F(k)$ , decaying as  $\exp(-\lambda z)$  at large positive  $z$ , with  $\lambda = \sqrt{-2\epsilon_b}$  and  $\epsilon_b = \Delta V + k^2/2$ . At large negative  $z$ , the latter functions are normalized as  $\sin(kz - \gamma)/\sqrt{\pi}$ . The functions associated with  $+k$  and  $-k$  are identical.

We introduce a background density of positive charges,  $n_0^+(z)$ , equal to the density of negative charges so that the sum of the Hartree potential,  $v_H$ , and the potential between positive and negative charges,  $v_+$ , is zero. Then we calculate the density, which involves the solution of the Kohn-Sham equation. The density is expressed as:

$$n_0(z) = 4 \int_0^{k_1^m} dk_1 |F(k_1)|^2 + 2 \int_{k_1^m}^{k_1^F} dk_1 |A_1(k_1)|^2 + 2 \int_0^{k_2^F} dk_2 |B_2(k_2)|^2 \quad (2.27a)$$

$$= 4 \int_0^{k_1^m} dk_1 |F(k_1)|^2 + 2 \int_0^{k_2^F} dk_2 \left[ \frac{k_2}{k_1} |A_1(k_1)|^2 + |B_2(k_2)|^2 \right] \quad (2.27b)$$

where  $(k_1^m)^2/2 = -\Delta V$ . In the second integral of (2.27b),  $k_1 = \sqrt{k_2^2 - 2\Delta V}$ . Results are given in Fig. 2.6 for two cases: (a)  $z_s^1 = 1$ ,  $z_s^2 = 2$  and (b)  $z_s^1 = 1$ ,  $z_s^2 = 1000$ .

## 2.2.2 Adiabatic force, energy-loss and friction

The asymmetry of the step potential has two consequences. On the one hand, the electrons exert a force on the step potential when it is at rest. If we move the step potential at vanishingly small velocities toward positive  $z$ , a finite energy is gained depending only on the displacement. This energy gain is lost when moving backward toward the initial position. On the other hand, for a finite velocity, the jellium is subject to a dissipative process which is proportional to the absolute value of the velocity (independently of its orientation) in the limit of small velocities. We set to establish these properties quantitatively.

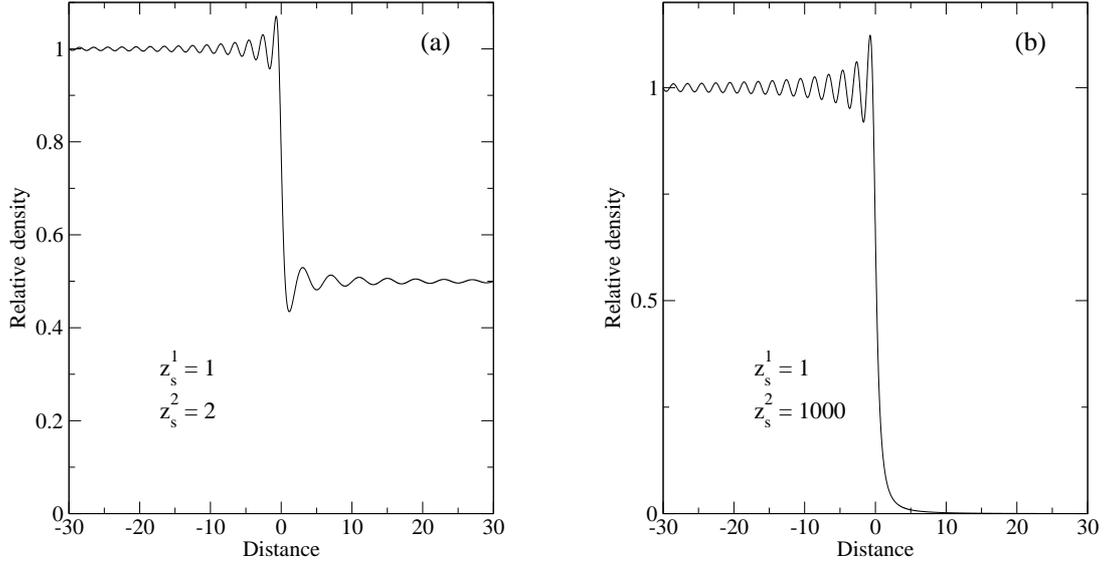

Figure 2.6: Density in the presence of a background potential (2.26) with  $z_1 = -0.5$ ,  $z_2 = 0.5$ ,  $z_s^1 = 1$  and (a)  $z_s^2 = 2$  or (b)  $z_s^2 = 1000$ . The density has been divided by the density of a uniform jellium with  $z_s = 1$ .

### Adiabatic force

**Electrons incident from  $+\infty$ :** The number of particles, with incoming momentum  $-k_2$ , reflected per unit time is  $k_2 P_r/2\pi$ , as can be verified by evaluating the current (1.9). If the step potential moves with velocity  $v$ , the energy transferred to the potential is  $-2k_2 v$ . The number of transmitted particles per unit time is  $k_2 P_t/2\pi$  and they transfer the energy  $(k_1 - k_2)v$ . Here, the reflection probability,  $P_r$ , and the transmission probability,  $P_t = 1 - P_r$ , are calculated for a given energy  $k_1^2/2 = k_2^2/2 + \Delta V$ . Therefore, the force on the potential is:

$$\frac{dE_2}{dz} = \frac{1}{2\pi} [(k_1 - k_2)k_2 P_t - 2k_2^2 P_r] \quad (2.28a)$$

$$= \frac{1}{2\pi} [k_2(k_1 - k_2) - k_2(k_1 + k_2) P_r] \quad (2.28b)$$

**Electrons incident from  $-\infty$  for positive energies:** The derivation is similar and yields:

$$\frac{dE_1}{dz} = \frac{1}{2\pi} [(k_1 - k_2)k_1 P_t + 2k_1^2 P_r] \quad (2.29a)$$

$$= \frac{1}{2\pi} [k_1(k_1 - k_2) + k_1(k_1 + k_2) P_r] \quad (2.29b)$$

**Electrons incident from  $-\infty$  for negative energies:** All electrons are reflected and give to the potential the energy  $2k_1 v$ . For a given  $k_1$ , the number of these reflected particles, per unit time, is,  $k_1/4\pi$  in view of the normalization of  $F(k_1)$ . Indeed, the function being real, the total current (sum of incoming and outgoing current) is zero. The asymptotic wave function

Table 2.2: Adiabatic force and friction for the background potential,  $(v_{\text{step}} + v^+)$ , alone. For the adiabatic force, numerical results obtained with (2.32b) and (2.33) are equal. In the expression of the step potential (2.26)  $z_1 = -0.5$  and  $z_2 = 0.5$ .

|                     |          |           |          |         |          |
|---------------------|----------|-----------|----------|---------|----------|
| $z_s^1; z_s^2$      | 0.5 ; 1. | 0.75 ; 1. | 1. ; 1.5 | 1. ; 2. | 1. ; 10. |
| $dE_{\text{ad}}/dz$ | 5.76     | 1.13      | 0.58     | 0.72    | 0.82     |
| Friction (2.37b)    | 1.08     | 0.133     | 0.151    | 0.351   | 1.24     |
| Friction (2.40)     | 1.07     | 0.130     | 0.149    | 0.348   | 1.32     |

can be written:

$$\frac{1}{\sqrt{\pi}} \sin(k_1 z - \gamma) = \frac{1}{2i\sqrt{\pi}} [e^{ik_1 z - i\gamma} - e^{-ik_1 z + i\gamma}] \quad (2.30)$$

The coefficient of the incoming wave (term in  $ik_1 z$ ) being  $\exp(-i\gamma)/2i\sqrt{\pi}$ , the associated current is  $k_1/4\pi$ . Finally the force on the potential is:

$$\frac{dE'_1}{dz} = \frac{1}{2\pi} k_1^2 \quad (2.31)$$

We now integrate over  $\mathbf{k}$  to get the total force on the potential (for two spin states):

$$\frac{dE_{\text{ad}}}{dz} = 2 \left[ 2 \int_0^{k_1^m} dk_1 \frac{dE'_1}{dz} + \int_{k_1^m}^{k_1^F} dk_1 \frac{dE_1}{dz} + \int_0^{k_2^F} dk_2 \frac{dE_2}{dz} \right] \quad (2.32a)$$

$$= \frac{2}{3\pi} [(k_1^F)^3 - (k_2^F)^3] \quad (2.32b)$$

Alternatively, the adiabatic force may be calculated in an obvious way from the average value of the potential derivative:

$$\frac{dE_{\text{ad}}}{dz} = \int_{-\infty}^{+\infty} dz n_0(z) \frac{dv_{\text{step}}}{dz} \quad (2.33)$$

since  $v_H + v_+ = 0$ . Results are given in Table 2.2.

### 2.2.3 Shifted Fermi surface

We now consider that the background potential is moving with velocity  $v$ . We must consider two possible cases.

$v < k_2^F$ : Then the expression of the density is:

$$n_v(z) = 4 \int_0^{k_1^m} dk_1 |F(k_1)|^2 + 2 \int_{k_1^m}^{k_1^F - v} dk_1 |A_1(k_1)|^2 + 2 \int_0^{k_2^F + v} dk_2 |B_2(k_2)|^2 \quad (2.34)$$

$v > k_2^F$ :

$$n_v(z) = 4 \int_0^{k_1^m - v} dk_1 |F(k_1)|^2 + 2 \int_0^{k_2^F + v} dk_2 |B_2(k_2)|^2 \quad (2.35)$$

## Friction

The friction coefficient is the linear term in  $v$  when calculating the difference between the energy change, per unit path length, for a velocity  $v$  and the adiabatic energy change. Again we have to consider two different situations:

- (i)  $v < k_2^F$ : Then the expression of the energy change is (for two spin states):

$$\frac{dE_v}{dz} = 2 \left[ 2 \int_0^{k_1^m} dk_1 \frac{dE'_1}{dz} + \int_{k_1^m}^{k_1^F - v} dk_1 \frac{dE_1}{dz} + \int_0^{k_2^F + v} dk_2 \frac{dE_2}{dz} \right] \quad (2.36a)$$

$$= 2 \left[ \frac{dE_{\text{ad}}}{dz} + \int_{k_1^F}^{k_1^F - v} dk_1 \frac{dE_1}{dz} + \int_{k_2^F}^{k_2^F + v} dk_2 \frac{dE_2}{dz} \right] \quad (2.36b)$$

A straightforward algebra leads to the result:

$$F = \lim_{v \rightarrow 0} \frac{1}{v} \left[ \frac{dE_v}{dz} - \frac{dE_{\text{ad}}}{dz} \right] = 2 \left[ - \left. \frac{dE_1}{dz} \right|_{k_1=k_1^F} + \left. \frac{dE_2}{dz} \right|_{k_2=k_2^F} \right] \quad (2.37a)$$

$$= -\frac{1}{\pi} \left[ (k_1^F)^2 - (k_2^F)^2 + (k_1^F + k_2^F)^2 P_r^F \right] \quad (2.37b)$$

where  $P_r^F$  is the reflection probability at the Fermi level. As for the case of the homogenous jellium, it can be shown that the latter expression is correct to first order in  $v$  when using the reflection probability calculated for the static case. Obviously, for  $k_1 = k_2$  we regain the result (2.23b)

- (ii)  $v > k_2^F$ : Calculating the limit for  $v$  tending to zero only makes sense if  $k_2^F$  is at least of order  $v^2$ , i.e., we may assume that  $k_2^F = 0$ . This corresponds to the case when the step potential models a surface. Then:

$$\frac{dE_v}{dz} = \frac{dE_{\text{ad}}}{dz} + 2 \int_{k_1^F}^{k_1^F - v} dk_1 \frac{dE'_1}{dz} + \int_0^v dk_2 \frac{dE_2}{dz} \quad (2.38)$$

so that

$$F = \lim_{v \rightarrow 0} \frac{1}{v} \left[ \frac{dE_v}{dz} - \frac{dE_{\text{ad}}}{dz} \right] = \frac{1}{\pi} \left[ -2(k_1^F)^2 + k_2^F(k_1^F - k_2^F) - k_2^F(k_1^F + k_2^F) P_r^F \right] \quad (2.39)$$

Alternatively, the friction coefficient may be calculated directly from the density of the SFS calculation. In doing that, we have to take into account that both the step potential and the potential due to the background of positive charges,  $v_+$ , move with the velocity  $v$ . Therefore:

$$F = \lim_{v \rightarrow 0} \frac{1}{v} \int_{-\infty}^{+\infty} dz [n_v(z) - n_0(z)] \left. \frac{d}{dZ} \right|_{Z=0} \left[ v_{\text{step}}(z - Z) + v_+(z - Z) \right] \quad (2.40)$$

Results are given in Table 2.2.

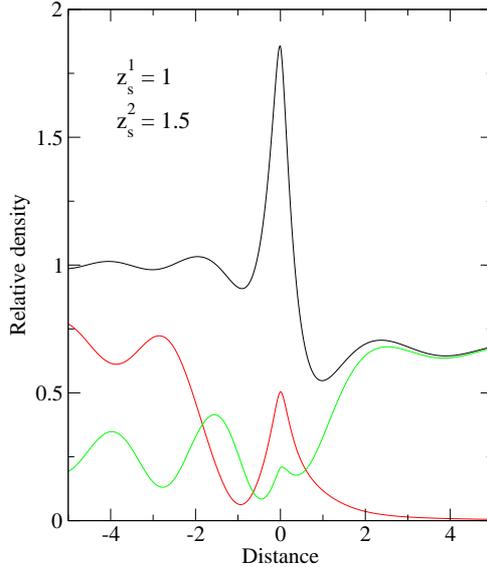

Figure 2.7: Density for an impurity in an inhomogeneous jellium. The background potential is defined by (2.26) with  $z_1 = -0.5$ ,  $z_2 = 0.5$ ,  $z_s^1 = 1$  and  $z_s^2 = 1.5$ . The density has been divided by the density of a uniform jellium with  $z_s = 1$ . Black curve: total density; red curve: contribution of the continuum with negative energy; green curve: contribution of the continuum with positive energies.

## 2.2.4 Impurity in an inhomogeneous jellium

### Static case

We now introduce an impurity, centered at  $z=0$ , as for the case of the homogenous jellium. Note that the position of the impurity with respect to the step potential may be changed at will by changing  $z_1$  and  $z_2$  in (2.26). In addition to the impurity, our model includes, as in the last section, a step potential and a background of positive charges with density  $n_0^+(z)$ . The expression of the density is the same as in (2.27b), except that we have to add the contribution of the bound state(s), as in (2.16). Results are given in Fig. 2.7 and Fig. 2.8 for the same impurity as in Section 2.1.2. With the parameters of Fig. 2.7,  $\Delta V = -0.685$  and there is one doubly occupied bound state with energy  $-0.764$ , i.e.,  $0.079$  below the band bottom. This proximity with the band bottom explains the presence of a peak in the contribution of the continuum with negative energies. In terms of a tight-binding language, this means that the bound state interacts with the nearby continuum. Note that  $v_{\text{step}}$  is equal to  $-0.342$  at  $z = 0$  and that the energy of the bound state for the homogenous case and  $z_s = 1$  is  $-0.410$ .

We note that the adiabatic force is unchanged with respect to the static case since (2.32b) does not involve the reflexion probability.

### Shifted Fermi Surface

The SFS calculations are formally identical to those carried out in the absence of an impurity. Results for the density are illustrated in Fig. 2.9.

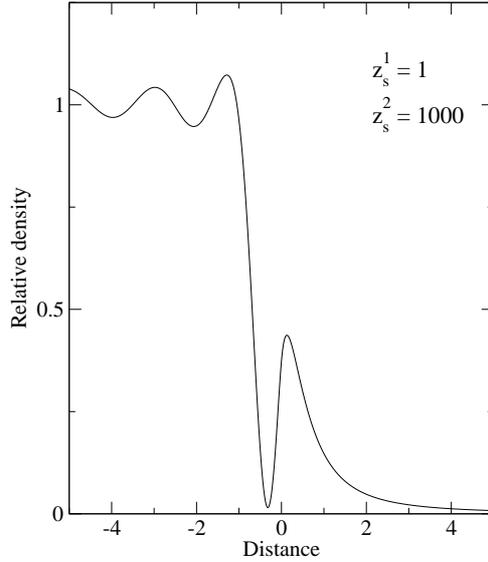

Figure 2.8: Density for an impurity in an inhomogeneous jellium. The background potential is defined by (2.26) with  $z_1 = -0.5$ ,  $z_2 = 0.5$ ,  $z_s^1 = 1$  and  $z_s^2 = 1000$ . The density has been divided by the density of a uniform jellium with  $z_s = 1$ . The bound state occupancy,  $m_b$ , has been set to zero, so that a resonance appears close to the band bottom which explains the presence of the bump close to the origin.

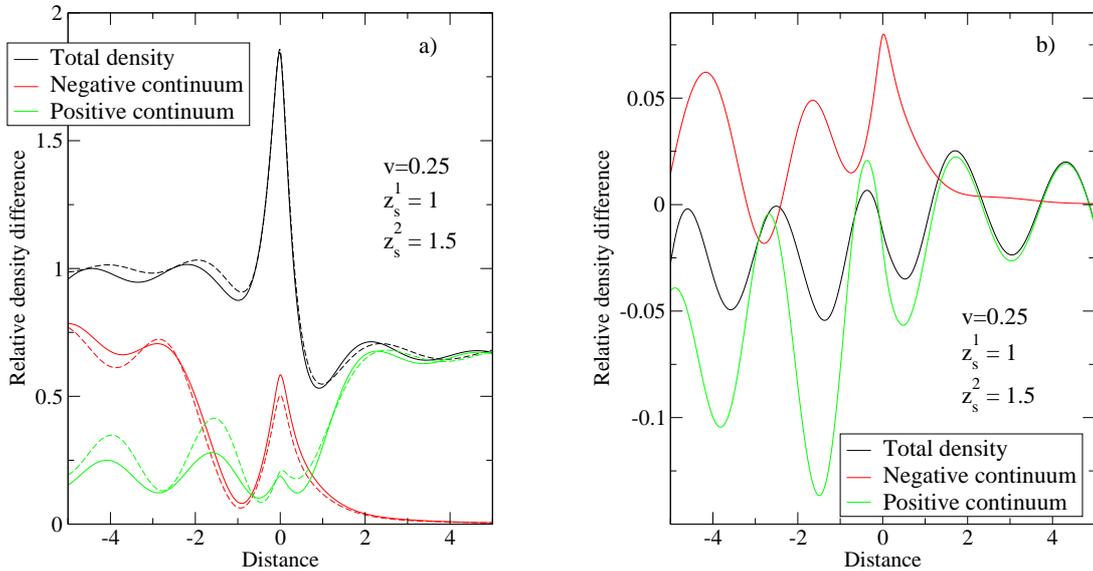

Figure 2.9: (a) Density and (b) density change for an impurity moving in an inhomogeneous jellium with a velocity  $v = 0.25$ . Other parameters are as in Fig. 2.7. Results have been divided by the density of a homogenous jellium for  $z_s = 1$ . Black curves: total density; red curve: contribution of the continuum for negative energies; green curve: contribution of the continuum with positive energies. The dashed curves give the results for the static case.

Table 2.3: Stopping power and friction coefficient for the impurity and background potential moving together. The stopping power estimated from (2.41) as a function of velocity is fitted by  $a_0v + a_1v^2 + a_2v^3$ . Results on the last line are evaluated from (2.37b). Results for (1;1.5) and (0.75;1) are for a double occupancy of the bound state and for (1;2) and (1;5) for single occupancy. Calculations are done for  $z \in [-5, 5]$  and  $\Delta z = 0.01$ .

| v                 | 0.75 ; 1     | 1 ; 1.5      | 1 ; 2        | 1 ; 5       |
|-------------------|--------------|--------------|--------------|-------------|
| 0.005             | —            | —            | —            | 0.00534     |
| 0.01              | 0.00578      | 0.00473      | 0.00548      | 0.0107      |
| 0.015             | —            | —            | —            | 0.0162      |
| 0.02              | 0.0116       | 0.00947      | 0.0110       | 0.0217      |
| 0.025             | —            | —            | —            | 0.0274      |
| 0.03              | 0.0174       | 0.0143       | 0.0166       | 0.0333      |
| 0.04              | 0.0233       | 0.0191       | 0.0223       | 0.0471      |
| 0.05              | 0.0293       | 0.0240       | 0.0281       | 0.0615      |
| 0.06              | 0.0354       | 0.0290       | 0.0341       | —           |
| 0.07              | 0.0417       | 0.0341       | 0.0403       | —           |
| 0.08              | 0.0480       | 0.0394       | 0.0466       | —           |
| 0.09              | 0.0546       | 0.0448       | 0.0532       | —           |
| 0.1               | 0.0613       | 0.0503       | 0.0600       | —           |
| $\underline{a_0}$ | <u>0.576</u> | <u>0.472</u> | <u>0.545</u> | <u>1.06</u> |
| $a_1$             | 0.051        | 0.018        | 0.148        | 0.03        |
| $a_2$             | 3.142        | 2.926        | 4.03         | 70.7        |
| Friction (2.37b)  | <u>0.573</u> | <u>0.466</u> | <u>0.546</u> | <u>1.07</u> |

## Friction coefficient

**Impurity and background potential moving together** As expression (2.37b) involves the reflexion probability for the full potential, it is still valid when both the impurity and background potential move together. The extension of (2.40) requires to include all those terms in the potential that are explicitly dependent on time. So, to first order in the velocity, the friction coefficient is:

$$F = \lim_{v \rightarrow 0} \frac{1}{v} \int_{-\infty}^{+\infty} dz [n_v(z) - n_0(z)] \left. \frac{d}{dZ} \right|_{Z=0} \left[ v_{\text{imp}}(z - Z) + v_{\text{step}}(z - Z) + v_+(z - Z) \right] \quad (2.41)$$

Results are given in Table 2.3.

**Impurity moving against fixed background** Expression (2.37b) is no longer valid and the expression of the friction coefficient is now:

$$F = \lim_{v \rightarrow 0} \frac{1}{v} \int_{-\infty}^{+\infty} dz [n_v(z) - n_0(z)] \left. \frac{d}{dZ} \right|_{Z=0} v_{\text{imp}}(z - Z) \quad (2.42)$$

Results are given in Table 2.4.

Table 2.4: Stopping power for the impurity moving in the inhomogeneous jellium created by the fixed background potential. The stopping power estimated from (2.42) as a function of velocity is fitted by  $a_0v + a_1v^2 + a_2v^3$ . Results for (1;1.5) and (0.75;1) are for a double occupancy of the bound state and for (1;2) and (1;5) for single occupancy. Calculations are done for  $z \in [-5, 5]$  and  $\Delta z = 0.01$ .

| v                 | 0.75 ; 1     | 1 ; 1.5      | 1 ; 2        | 1 ; 5       |
|-------------------|--------------|--------------|--------------|-------------|
| 0.05              | —            | —            | —            | 0.00358     |
| 0.01              | 0.00326      | 0.00462      | 0.00445      | 0.0072      |
| 0.015             | —            | —            | —            | 0.0109      |
| 0.02              | 0.0662       | 0.00931      | 0.00899      | 0.0146      |
| 0.025             | —            | —            | —            | 0.0185      |
| 0.03              | 0.0101       | 0.0141       | 0.0137       | 0.0225      |
| 0.04              | 0.0137       | 0.0190       | 0.0185       | 0.0320      |
| 0.05              | 0.0174       | 0.0240       | 0.0235       | 0.0420      |
| 0.06              | 0.0212       | 0.0292       | 0.0286       | —           |
| 0.07              | 0.0253       | 0.0345       | 0.0340       | —           |
| 0.08              | 0.0295       | 0.0400       | 0.0397       | —           |
| 0.09              | 0.0339       | 0.0457       | 0.0456       | —           |
| 0.1               | 0.0385       | 0.0515       | 0.0518       | —           |
| $\underline{a_0}$ | <u>0.321</u> | <u>0.458</u> | <u>0.440</u> | <u>0.71</u> |
| $a_1$             | 0.434        | 0.302        | 0.4          | 0.001       |
| $a_2$             | 2.02         | 2.67         | 3.88         | 52.9        |

## 2.2.5 Expression of Helsing and Persson

### Reduction from 3D to 1D

We wish to derive the expression of Helsing and Persson for the 1D case. Their expression for the 3D case is given by Eq. 23 of [2]. To avoid any mistake, we proceed with the reduction from 3D to 1D of the SFS friction coefficient for a homogenous jellium. We should regain expression (2.23b). We start with Eq. 22 of Supplemental [2]:

$$\Gamma_{\text{SFS}}(3\text{D}) = 4\pi k_F^4 \int d\hat{\mathbf{k}}_F \int d\hat{\mathbf{k}}'_F \cos \theta_{k_F} [\hat{\mathbf{v}} \cdot (\hat{\mathbf{k}}_F - \hat{\mathbf{k}}'_F)] \left| \int d\mathbf{r} [\phi_{\mathbf{k}'_F}(\mathbf{r})]^* V_0(\mathbf{r}) \psi_{\mathbf{k}_F}^+(\mathbf{r}) \right|^2 \quad (2.43)$$

The shift from 3D to 1D involves the following changes:

- Change in function norms:  $(2\pi)^{-3/2}$  in 3D and  $(2\pi)^{-1/2}$  in 1D  $\rightarrow$  factor  $(2\pi)^4$ .
- No angular integral  $\rightarrow$  factor  $(2\pi)^{-4}$  (NB:  $2\pi$  and not  $4\pi$  because, in 1D, we integrate over positive and negative  $\mathbf{k}$ ).
- The differential element in the  $\mathbf{k}_F$  integration does not involve  $k_F^2 \rightarrow$  factor  $k_F^{-4}$ .
- For a given value of  $\mathbf{k}_F$ , the only contribution is for  $\mathbf{k}'_F = -\mathbf{k}_F$  and the term  $\hat{\mathbf{k}}_F - \hat{\mathbf{k}}'_F$  is equal to 2. As there are two possible values of  $\mathbf{k}_F$ , we get globally a factor of 4.

We end with:

$$\Gamma_{\text{SFS}}(1\text{D}) = 16\pi \left| \int_{-\infty}^{+\infty} dz [\phi_{k_F}(z)]^* V_0(z) B_{k_F}(z) \right|^2 \quad (2.44)$$

Now if we substitute in (2.23b) expression (1.26) for  $P_r = |F_r|^2$  and  $k_1 = k_2$ , we get exactly (2.44), which confirms the validity of our procedure.

We now turn to the 3D formula of Helsing and Persson (Eq. 23 of [2]):

$$\Gamma_{\text{HP}}(3\text{D}) = 2\pi \int d\mathbf{k} \int d\mathbf{k}' \left| \int d\mathbf{r} [\psi_{\mathbf{k}'}^-(\mathbf{r})]^* \frac{dV_0}{dQ} \psi_{\mathbf{k}}^+(\mathbf{r}) \right|^2 \delta(\epsilon_F - \epsilon_k) \delta(\epsilon_F - \epsilon_{k'}) \quad (2.45)$$

The shift from 3D to 1D involves the following changes:

- Change in function norms:  $(2\pi)^{-3/2}$  in 3D and  $(2\pi)^{-1/2}$  in 1D  $\rightarrow$  factor  $(2\pi)^4$ .
- No angular integral  $\rightarrow$  factor  $(2\pi)^{-4}$ .

The final result is:

$$\Gamma_{\text{HP}}(1\text{D}) = 2\pi \int d\mathbf{k} \int d\mathbf{k}' \left| \int dz [\psi_{\mathbf{k}'}^-(z)]^* \frac{dV_0}{dz} \psi_{\mathbf{k}}^+(z) \right|^2 \delta(\epsilon_F - \epsilon_k) \delta(\epsilon_F - \epsilon_{k'}) \quad (2.46)$$

We may check that the coefficient is correct by making calculations for the homogenous case since we know that  $\Gamma_{\text{HP}}$  is correct in the latter case.

## Calculation of $\Gamma_{\text{HP}}$

The 3D distinction between ingoing and outgoing waves, represented by the + and – labels, makes no sense in 1D though we have been using the same terminology to distinguish wavefunctions for positive and negative values of  $\mathbf{k}$ . We have already noted that a positive  $\mathbf{k}$  is associated with a  $B_{k_2}$  function and a negative  $\mathbf{k}$  with a  $A_{k_1}$  function. Making this relation explicit, we get:

$$\begin{aligned} \Gamma_{\text{HP}} = & 2\pi \left\{ \int_0^\infty dk_1 \int_0^\infty dk'_1 \left| \int dz [A_{k'_1}(z)]^* \frac{dV_0}{dz} A_{k_1}(z) \right|^2 \delta(\epsilon_F - \epsilon_{k'_1}) \delta(\epsilon_F - \epsilon_{k_1}) \right. \\ & + \int_0^\infty dk_2 \int_0^\infty dk'_2 \left| \int dz [B_{k'_2}(z)]^* \frac{dV_0}{dz} B_{k_2}(z) \right|^2 \delta(\epsilon_F - \epsilon_{k'_2}) \delta(\epsilon_F - \epsilon_{k_2}) \\ & \left. + 2 \int_0^\infty dk_1 \int_0^\infty dk_2 \left| \int dz [A_{k_1}(z)]^* \frac{dV_0}{dz} B_{k_2}(z) \right|^2 \delta(\epsilon_F - \epsilon_{k_1}) \delta(\epsilon_F - \epsilon_{k_2}) \right\} \quad (2.47) \end{aligned}$$

Integrating over  $k$ 's:

$$\begin{aligned} \Gamma_{\text{HP}} = & 2\pi \left\{ \frac{1}{(k_1^F)^2} \left| \int dz [A_{k_1^F}(z)]^* \frac{dV_0}{dz} A_{k_1^F}(z) \right|^2 \right. \\ & + \frac{1}{(k_2^F)^2} \left| \int dz [B_{k_2^F}(z)]^* \frac{dV_0}{dz} B_{k_2^F}(z) \right|^2 \\ & \left. + \frac{2}{k_1^F k_2^F} \left| \int dz [A_{k_1^F}(z)]^* \frac{dV_0}{dz} B_{k_2^F}(z) \right|^2 \right\} \quad (2.48) \end{aligned}$$

As a check of our numerical methods, we may calculate the friction coefficient when the projectile moves together with the background potential. In the latter case, it can be shown that (2.48) is equivalent to (2.37b). We first note that, for a given initial state in (2.48), a sum is carried out over the two final degenerate states. Any complete set can be used within this subspace, which allows us to replace the set  $A_{k_1^F}^*, B_{k_2^F}^*$  by  $A_{k_1^F}, B_{k_2^F}$  (a claim that we have checked numerically). We are, then, in a position to use (1.33) and (1.34). The proof follows the same line as that given in Section 5 of Ref. [2]. On the one hand, expression (2.37b) can be transformed by using (1.26) and (1.27) in (2.28a) and (2.29a). On the other hand, a 1D transformation similar to Eq. (36) of [2] can be derived<sup>1</sup>. The latter point is the key one to prove the equivalence between  $\Gamma_{\text{HP}}$  and  $\Gamma_{\text{SFS}}$ : when the impurity potential moves with the background potential, the state of the system evolves from one point to the other through a mere translation.

Results for  $\Gamma_{\text{HP}}$  and  $\Gamma_{\text{SFS}}$  are given in Table 2.5. Within the accuracy of the calculations, they are equal.

---

<sup>1</sup>Here, in addition to the matrix element of  $V_0$ , one has to cope with additional terms as in (1.26) and (1.27).

Table 2.5: Friction coefficient for the impurity and background potential moving together. Results for (1;1.5) and (0.75;1) are for a double occupancy of the bound state and for (1;2) and (1;5) for a single occupancy. Calculations are done for  $z \in [-5, 5]$  and  $\Delta z = 0.01$

| $z_s^1 ; z_s^2$                    | 0.75 ; 1 | 1 ; 1.5 | 1 ; 2 | 1 ; 5 |
|------------------------------------|----------|---------|-------|-------|
| $\Gamma_{\text{SFS}}$ from (2.37b) | 0.573    | 0.466   | 0.546 | 1.07  |
| $\Gamma_{\text{HP}}$ from (2.48)   | 0.576    | 0.476   | 0.560 | 1.12  |

# Bibliography

- [1] C. Cohen-Tannoudji, B. Diu and F. Laloë, *Quantum mechanics* (Wiley-Interscience, New-York, 1977)
- [2] A. Salin, Note1.pdf of this Ancillary material.
